# Supplementary material for: Frequency and amplitude dependent population dynamics during cycles of feast and famine
Source: arXiv:1612.09330 ancillary file (2018-02-21)
Supplement: Supplementary file 1 [file Supplemental_Material.pdf]

# Supplemental Material for *Frequency and amplitude dependent population dynamics during cycles of feast and famine*

Jason Merritt[1,2] and Seppe Kuehn[1,2,3*]
[1] *Center for the Physics of Living Cells, University of Illinois at Urbana-Champaign, Urbana, IL 61801, USA.*
[2] *Department of Physics, University of Illinois at Urbana-Champaign, Urbana, IL 61801, USA.*
[3] *Center for Biophysics and Quantitative Biology, University of Illinois at Urbana-Champaign, Urbana, IL 61801, USA.*

## Supplementary Material: Experiments

### I. STRAINS AND GROWTH CONDITIONS

All liquid media used was M63 minimal media with 0.04% (w/v) glucose and $12.5\,\mu g\,mL^{-1}$ chloramphenicol. Plates were lysogeny broth (LB) plates, also with $12.5\,\mu g\,mL^{-1}$ chloramphenicol. Every phase of each experiment was carried out at 30 °C. Initial flask cultures were grown in shakers operating at 200 rpm, and all continuous-culture devices were constantly stirred at 800 rpm.

Our *Escherichia coli* strain was created by D. Hekstra at Rockefeller University: MG1655 $\Delta fimA$, $\Delta flu$, HK022 att:: ($catP_{\lambda R}$-*dTomato*) *hsdR*.

### II. LAG-TIME MEASUREMENT

To measure the lag-time for populations growing in our chemostat we followed a method described elsewhere [1]. Briefly, cells were sampled from chemostats and plated on LB agar plates. Plates were then incubated and continuously imaged. Image processing was used to determine the time to colony formation and the rate of colony growth.

#### A. Plate preparation protocol

We initially recorded considerable variability in our plating data due to the sensitivity of *E. coli* colonies to the conditions of the plate, such as initial temperature and water content due to evaporation and condensation. To standardize our methodology and ensure the consistency of our results, we developed the following protocol for preparing plates for imaging.

LB-agar (1.5 % w/v, with chloramphenicol) is poured at 50 °C into 100 mm diameter plates 10 days before the first plate is imaged, using a sterilized graduated cylinder to measure out 18 mL per plate. Shortly after solidifying, plates are inverted and left on a lab bench top at room temperature for 2 days, then individually sealed in parafilm and transferred to a refrigerator at 4 °C for 7 days, by which time the plates are assumed to have reached an environmental steady state. Starting on the $7^{\text{th}}$ day, plates are taken out of the refrigerator as needed 24 hours before they are scheduled to be imaged. The plates taken from the refrigerator have their parafilm removed and are placed in an incubator at 30 °C to thermalize at the temperature of the experiment for 24 hours. Finally, samples from the continuous-culture devices are spread onto these plates, and the plates are grown and imaged at 30 °C.

Plates were imaged every 5 or 10 minutes for 24 hours using a commercial webcam housed in a light tight box. An LED strip controlled by a relay was used to illuminate the plates only during imaging (~1 second for each acquisition).

#### B. Colony image processing

Depending on the experiment, an image of each plate was taken every 5 or 10 minutes. Circular regions of interest (ROIs) were determined by hand for each imaged plate [Fig. S1(b)]. These ROIs were background-subtracted using a median filter on at least 10 images, taken over a period of 100 minutes, before the first colonies appeared in any experiment [Fig. S1(c)], and were then globally thresholded using a fixed value across all experiments [Fig. S1(d)]. ROI size was controlled by hand to exclude light reflection artifacts near the edge of each plate without excluding any colonies on the plates.

For each thresholded image, SCIKIT-IMAGE functions were used to find and record all information about all connected regions above the threshold (including both colonies and artifacts). Next, detected objects appearing in the same location were associated across sequentially acquired images to allow size tracking in time. Since imaging artifacts do not persist across multiple images they are filtered out at this step. Finally, only colonies which did not merge with other colonies during growth are included in the final analysis, because colonies very near each other on the plate affect each others' growth. However, for colonies evenly distributed on a plate, previous work by Levin-Reisman *et al.* [1] showed no effect on the growth of neighboring colonies as long as the total number of colonies on the plate remained below 200. We stay below this threshold in our experiment.

* To whom correspondence should be addressed: seppe@illinois.edu

The first image in which a colony appeared was used to define its 'time to colony appearance' [Fig. S2(b)], which we found generally followed a normal distribution [Fig. S3]. Our data indicated that colony area increased linearly in time over the first 70 minutes of detection [Fig. S4]; therefore, the colony rate of area increase [Fig. S2(c)] was determined by a linear fit to the colony's size over the first 70 minutes after its appearance.

Because our plate illumination results in a background brightness gradient increasing radially from the center of the plate [Fig. S1(b)], we checked the time to colony appearance and colony growth rate in our experiment against the background brightness of their location on the plate [Fig. S5(a)] and found an increase in time to colony appearance and a decrease in colony growth rate for colonies growing in regions where the background intensity of the plate exceeds a pixel intensity of 100. Our reported qualitative trends for these variables, shown in Fig. S2, remain intact with these colonies discarded [Fig. S5(c)].

Total numbers of colonies were also counted by hand from the physical plates for statistics on cell viability over time [Fig. S6].

### C. Lag-time measurements: frequency dependence

Lag-time measurements were carried out as described above in chemostats with 1 h washout events at washout schedules of 24 h, 48 h, and 72 h, with multiple sampling times over a period of 72 h following the first washout event [Fig. S2(a)]. We observe an increase in lag-time - as measured via average time to colony appearance - with increasing duration of starvation [Fig. S2(b)].

### D. Lag-time measurements: amplitude dependence

Lag-time measurements were also carried out at a single point, 12 hours after the beginning of the first washout event, in systems undergoing 1 h, 1.5 h, and 2 h washout events [Fig. S7]. These experiments were carried out in a modified imaging apparatus that permitted higher throughput plate imaging. This resulted in different illumination profiles of the plates and therefore quantitative changes in the minimum detectable colony size. As a result, direct numerical comparisons to Fig. S2(b) are not possible, but the average times to colony appearance from this set of experiments indicates a decrease in lag time with increasing washout amplitude [Fig. S7].

## III. MEASUREMENTS OF SYSTEM DYNAMICS BY MICROSCOPY

### A. Recovery rate estimation

Spline fits are used to provide smoothed curves for estimating maximum growth rates during recovery (Figs. 1(c), 2(a), main text). Spline estimates for $N(t)$, the cell abundances as a function of time, were computed as detailed in Merritt & Kuehn 2016 [2], with spline estimates performed on raw (not rolling average) single-cell counts. Cubic splines returned an estimate of the number of single cells per image which we denote $\hat{N}(t)$. We performed these spline fits after each washout event for all of the data shown in Fig. 2 of the main text. To estimate the instantaneous growth rate we computed $\frac{d ln \hat{N}(t)}{dt}$.

### B. Cell aggregation

Our systems exhibit complex dynamics in the form of cell aggregation into large free-floating aggregates following the recovery after a washout event [2]. Statistics on aggregate abundances are complicated by very low abundances (~1 per image), and our estimated measured aggregate abundances do not appear to have a simple relationship with population recovery rates [Fig. S9], individual cell size [Fig. S8], or lag-phase [Fig. S10].

#### *1. Distributions and dynamics aggregate sizes*

We studied the distribution of object sizes for all objects detected by our image processing algorithm. We constructed binned probability histograms of the size of all objects detected during the 9 day experiment window, with logarithmic bins of object area and each bin normalized by the total number of objects. These histograms contained two peaks, one corresponding to planktonic cells and one corresponding to aggregates [Fig. S11]. From these histograms we note that the characteristic cross-sectional area of aggregates in our images is approximately 29 times greater than that of single cells - the latter have an average size (in the plane of focus) of approximately 4.15 µm$^2$ (135 pixels), with aggregates having a size of approximately 121 µm$^2$ (3910 pixels). This gives an estimate of the number of cell volumes contained in an aggregate volume of $(\frac{121}{4.15})^{1.5} = 157$ cell volumes per aggregate. Assuming a packing fraction (fraction of aggregate volume that is cells) of about 0.64 - typical for a close random packing of spheres - yields our rough estimate of approximately 100 cells per aggregate. These histograms also corroborate our claim that the batch-culture conditions ($D = 0$ between washout events) result in little or no aggregation.

We next studied the dynamics of aggregate sizes over time. To do this we constructed distributions of aggre-

gate area in the plane of focus for non-overlapping 3 hour time windows throughout the time series for all experiments. We then plotted the average of these distributions as a function of time and found that the average aggregate size decreased after washout events in all conditions [Fig. S12]. This observation strongly supports our modeling assumption that increases in nutrient levels drive aggregate dispersal.

#### 2. *Time series of aggregate abundances*

For completeness, we present representative aggregate abundance time series (smoothed with a rolling average) under 48 h washout periods (at washout durations of 1 h, 1.5 h, and 2 h) and a 72 h washout period (at a washout duration of 1 h) in Fig. S13. Representative aggregate abundance time series under 24 h washout periods for all washout durations are presented in Fig. 2(b) of the main text.

## IV. MEASUREMENTS OF SYSTEM DYNAMICS BY OPTICAL DENSITY

Our devices also record transmitted light intensity in real time during each experiment using a photodiode and infrared LED pair. These data permit us to measure abundance dynamics indirectly, and to corroborate our findings of frequency and amplitude dependent dynamics [Fig. S14(a)]. However, our optical density measurement is complicated by a varying optical density value for ‘zero’ abundance - the expected measurement if the vial were filled with water. This value fluctuates over the course of each experiment, most likely due both to changes in the density of biofilm on the vial walls and physical disturbance of the vial itself, which can rotate somewhat freely and is periodically lifted from the system during operation to check for system failure.

### A. Analysis of optical density data

To calculate the optical density recovery data shown in Fig. S14(a), we add an additional step to the spline-based recovery rate estimation mentioned above. Because growth during washout events is in general slow following hours of steady-state growth, we assume an exponential decay of the population during the brief washout period, and therefore use a decaying exponential fit during each washout to estimate the ‘zero’ abundance value the photodiode reading is asymptotically approaching [Fig. S14(b)]. This ‘zero’ abundance value is subtracted from the recovery immediately following the washout event to generate an adjusted time series that can be used to estimate recovery growth rates. Splines are then applied to these adjusted time series to estimate maximum rates of recovery via the same analysis used for single-cell counts.

This measurement corroborates the central claim of this paper with a measurement which is completely independent of our image acquisition and analysis, as shown by the similarity between Fig. S14(a) and Fig. 2(a) in the main text.

## V. ADDITIONAL EXPERIMENTS

### A. Repeated batch culture experiments

In addition to our standard continuous-culture experiments, consisting of standard chemostat operation interrupted by periods of rapid washout, we also performed several ‘batch’-style experiments. These repeated batch experiments, which can roughly be interpreted as simulating repeated inoculations from one batch culture to another, are identical to our standard experiments, but with a basal dilution rate of zero outside of the scheduled washout event periods. As aggregates do not typically form in our systems in when $D = 0$ (batch culture conditions) [Fig. S8(a)], we view these experiments as a test on the role of cell aggregates and the history-dependent recovery dynamics we observe when $D > 0$ between washout events. However, cells are too dim in these conditions for our image segmentation to reliably detect during all stages of growth. Because we found optical density recovery dynamics [Fig. S14(a)] displayed the same trends as single-cell abundance recovery dynamics (Fig. 2(a), main text), we instead relied on optical density measurements to analyze these ‘batch’-style experiments, which were carried out with 1 h and 2 h washout events at a 24 h washout period, and 1 h washout events at a 48 h washout period [Fig. S15(a)].

Unlike our standard continuous-culture experiments, the expected frequency-dependence and amplitude-dependence in recovery dynamics are essentially absent, except in the 2 h washout condition [Fig. S15(c)], where a fast recovery appears to correlate to the eventual arrival of aggregates in the system after 5 days [Fig. S15(b)].

These results show that the presence of aggregates are a necessary condition for the observation of fast recovery rates. They also suggest that higher average dilution rates drive aggregation, since we observe the formation of aggregates at late times in the 2 h condition. Our model does not include this phenomenon.

### B. High frequency washout events: 12 hour data

We also carried out a high-frequency washout continuous-culture experiment, with 1 h washouts every 12 h, chosen to be roughly the same amount of time it takes one of our continuous-culture populations to fully recover following a 1 h washout event. Our previous work [2] indicates the appearance of aggregates following a

washout event is correlated to the onset of slow growth occurring when the population of single-cells nears maximum density. Consistent with this, the aggregate abundances we detect fail to reach appreciable levels during the 9-day experimental window, as the appearance of cell aggregates is also immediately cut off by the next washout event [Fig. S16(b)]. However, the systems still maintain a fast growth rate during recovery [Fig. S16(a)], possibly due to sources of aggregation not visible to our microscope, e.g. wall growth. Our model cannot capture the dynamics at these very high frequencies [Fig. S17] for the simple reason that there is insufficient time for aggregates to form when washout events occur at high frequency. One possible reason for this discrepancy is that high frequency washout events may drive more substantial and rapid adhesion to the culture vessel itself (e.g., decrease $\rho$). At present we cannot quantitatively test this conjecture.

# Supplementary Material: Modeling

## VI. MODEL STRUCTURE

Here we recapitulate the model presented in the main text and provide motivation for the parameter values chosen in the numerical simulation presented in Fig. 3 of the main text. The model is as follows:

$$\dot{N} = \mu(S)N - DN - \alpha_1(1-f(S))N + \alpha_2\frac{Q}{1+Q}f(S)AY_{NA}, \quad (1)$$

$$\dot{A} = \alpha_1(1-f(S))\frac{N}{Y_{NA}} - \alpha_2\frac{Q}{1+Q}f(S)A - \rho DA, \quad (2)$$

$$\dot{S} = (S_r - S)D - \frac{\mu(S)}{y}N, \quad (3)$$

$$\dot{Q} = \begin{cases} aQ & S \geq S_c \\ -bQ & S < S_c \end{cases}, \quad (4)$$

$$f(S) = \begin{cases} 0 & S \leq S_{th} \\ \frac{S-S_{th}}{S_r-S_{th}} & S > S_{th} \end{cases}, \quad (5)$$

$$\mu(S) = \frac{\mu_m S}{K+S}. \quad (6)$$

$N$ is the abundance of planktonic cells, $A$ is the abundance of aggregated or adherent cells, $S$ is the substrate (glucose) concentration, $Y_{NA}$ is the number of cells per aggregate, $D$ is the dilution rate of the chemostat, $\alpha_1$ is the rate of formation of aggregates, $\alpha_2$ is the rate of dispersal of aggregates, $0 \leq \rho \leq 1$ simulates the role of adherent populations not washed out of the system, $y$ is the yield of bacteria on the substrate, $S_c$ and $S_{th}$ are parameters.

Note that in the simulation we set $y = 1$ and $S_r = 100$ without loss of generality. Experimentally, $S_r = 2.2$mM which yields a maximum cell density of approximately $5 \times 10^8$ cells/mL. We perform simulations over a range of $S_c$, $S_{th}$, and $\rho$ to test the sensitivity of our conclusions to these unknown parameters. The results are shown in Fig. S18. We find little sensitivity of our conclusions to changes in $S_c$ and $S_{th}$, but stronger sensitivity to the value of $\rho$.

Below we present the value of each parameter used in the simulation and a justification.

TABLE I. Model parameter values

| Parameter | value | justification |
|---|---|---|
| $\mu_m$ | $0.3\,\mathrm{h}^{-1}$ | [3] |
| $K$ | 45 $\mu$M | [4] |
| $\alpha_1$ | $0.04\,\mathrm{h}^{-1}$ | inferred |
| $\alpha_2$ | $0.125\,\mathrm{h}^{-1}$ | see below |
| $Y_{NA}$ | 100 cells/aggregate | Fig. S11 |
| $a$ | $0.07\,\mathrm{h}^{-1}$ | see below |
| $b$ | $0.0275\,\mathrm{h}^{-1}$ | see below |
| $S_c$ | 0.22 mM | see below |
| $S_{th}$ | 1.5 mM | see below |
| $\rho$ | 0.1 | see below |

### A. Bounds on $\alpha_1$ and $\alpha_2$

Direct measurement of aggregation/adherence and dispersal rates in our experiment is not possible. However, from general considerations we can place some bounds on what these rates ($\alpha_1$ and $\alpha_2$) should be. We begin by considering the limit where $S << S_{th}$. In this case, growth is slow and the equations describing $N$ and $A$ become

$$\dot{N} = \mu(S)N - (D + \alpha_1)N, \quad (7)$$

$$\dot{A} = \alpha_1\frac{N}{Y_{NA}} - \rho DA. \quad (8)$$

Aggregation then acts to increase the effective planktonic dilution rate by $\alpha_1$. This reduces the steady state abundance of planktonic cells in the system ($N^*$), which is a declining function of $D$. Experimentally we observe a decline in the planktonic abundances as the aggregation process proceeds after a washout event (for example, see Fig. 1 in the main text and Fig. S8(b)). This decline is on the order of 20 % of the maximum planktonic abundances we observe. By simulating the $S << S_{th}$

limit we find that for $D = 0.08\,\mathrm{h}^{-1}$, $\alpha_1 = 0.04\,\mathrm{h}^{-1}$ results in a roughly 20 % decline in steady state planktonic abundances due to aggregation. We therefore fix $\alpha_1$ to $0.04\,\mathrm{h}^{-1}$ for all simulations presented here (Table I).

Next we consider the limit where $f(S) = 1$ ($S \to S_r$) and ask how big an effect on the planktonic population growth rate the dispersal of $A$ can have. To estimate this we consider the case where $f(S) = 1$ and $Q >> 1$:

$$\dot{N} = \mu_m N - DN + \alpha_2 A Y_{NA}. \tag{9}$$

Rewriting the density of the $A$ population by $N_A = AY_{NA}$ and dividing through by $N$ we get

$$\frac{dln(N)}{dt} = \mu_m - D + \alpha_2 \frac{N_A}{N}. \tag{10}$$

For dispersal to have an appreciable impact on the planktonic population growth rate we require that $\mu(S) \approx \alpha_2 \frac{N_A}{N}$ which requires either an $A$ population which dramatically exceeds $N$ or a dispersal rate that is of the same order as $\mu_m$. From our measurement of the aggregate densities (Fig. 1, main text) and the average size of aggregates [Fig. S11] we assume that the ratio $\frac{N_A}{N}$ is of order 1 to 10, which suggests that the dispersal rate must be of order $\mu_m$. We choose a value for this parameter which satisfies this constraint (Table I).

### B. Values of $S_c$ and $S_{th}$

$S_{th}$ sets the substrate level controlling dispersal. We note that neither of these parameters are known. However, we do know that aggregation appears to increase substantially as growth rates slow during a recovery [2]. Further, given the amplitude dependence of the recovery rate we observe in experiment (Fig. 2(a), main text) the dispersal rate of $A$ should be sensitive to the substrate concentration in the neighborhood of 2 mM. Within these constraints we find that a wide range of values for $S_{th}$ recapitulate our observations [Fig. S18].

Although the processes regulating biofilm maturation in *E. coli* are complex, gene expression levels suggests the presence of effectively starved, stationary-phase cells may be necessary for biofilm maturation, and that penetration of nutrients into biofilms may directly hinder their formation [5]. For our model, we extend this idea to external substrate levels - assuming the amount of substrate penetrating into biofilms rises in proportion to rising external substrate levels - through the parameter $S_c$, which explicitly sets the substrate level at which the maturation process proceeds (or degrades). $S_c$ is chosen to be substantially smaller than $S_{th}$ as it is assumed to directly relate to nutrient limitation, but a similarly wide range of values of $S_c$ reproduce our results [Fig. S18].

### C. Value of $\rho$

In our model $\rho$ is a proxy for the reduced effect of dilution on aggregated cells due to adherence to the wall; $\rho = 1$ would indicate a fully free-floating aggregate population, and $\rho = 0$ would indicate an entirely adherent population. While we cannot measure $\rho$ directly, simulations over a range of values show that our results are sensitive to the choice of $\rho$ [Fig. S18]. We note that at $\rho \approx 1$ we fail to observe the strong amplitude and frequency dependence in simulation that we observed in experiment, and therefore conclude that some adherent populations are necessary to account for our results. Past this, $\rho$ was chosen as a free parameter; however, as discussed above, our model cannot capture the experimental dynamics at very high frequencies [Fig. S17], which may imply a decrease in $\rho$ (increased adherence) in rapid washout conditions.

### D. Dynamics of $Q$: rates $a$ and $b$

In our model of abundance dynamics the frequency dependence results from a declining rate of dispersal for the $A$ population as the duration of famine increases. This process - biofilm maturation - is described by the variable $Q$. When $Q$ is small (long periods of $S < S_c$) the dispersal rate is proportional to $Q$. Conversely, when $Q$ is large, dispersal is independent of this internal variable. The dynamics of $Q$ are assumed to be autocatalytic (see main text) with rates $a$ and $b$. In the 72 hour condition long periods of famine result in small $Q$ and limited dispersal and therefore slow recoveries. In the 24 hour condition we observe fast recoveries driven by $A$ dispersal because $Q >> 1$. Therefore, we set the values of $a$ and $b$ in our simulation (Table I) such that $Q < 1$ for a 72 hour cycle and $Q >> 1$ for a 24 hour cycle.

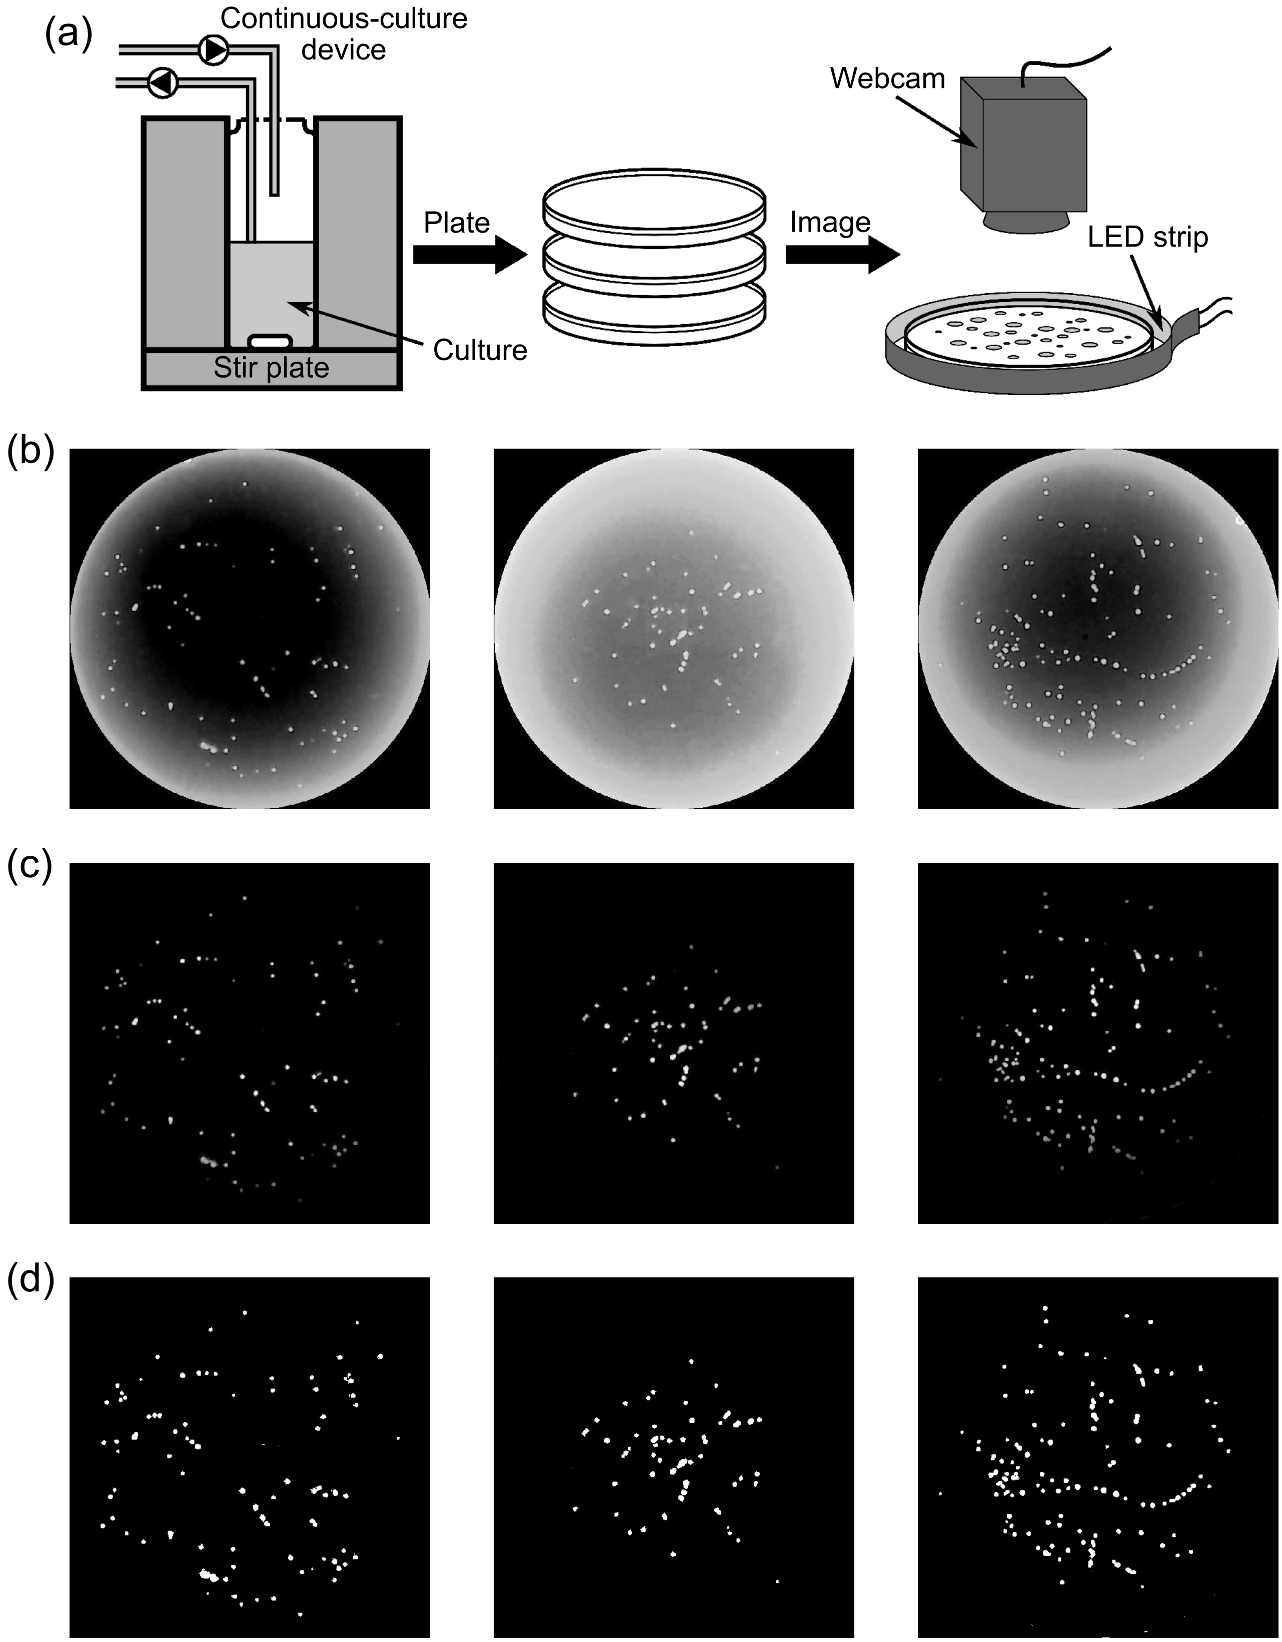


FIG. S1. Plate imaging technique. (a) Schematic of the measurement. Cells are sampled manually from a chemostat and plated. A webcam images plates housed in an environmental chamber maintained at 30 °C. (b) Circular regions of interest (ROIs) from images of three example plates. Note that intensity increases towards plate boundaries due to plates being lit from the sides by LED strips. (c) Background-subtracted versions of the images shown in (a). (d) Thresholded versions of the images shown in (b), showing detected colonies.

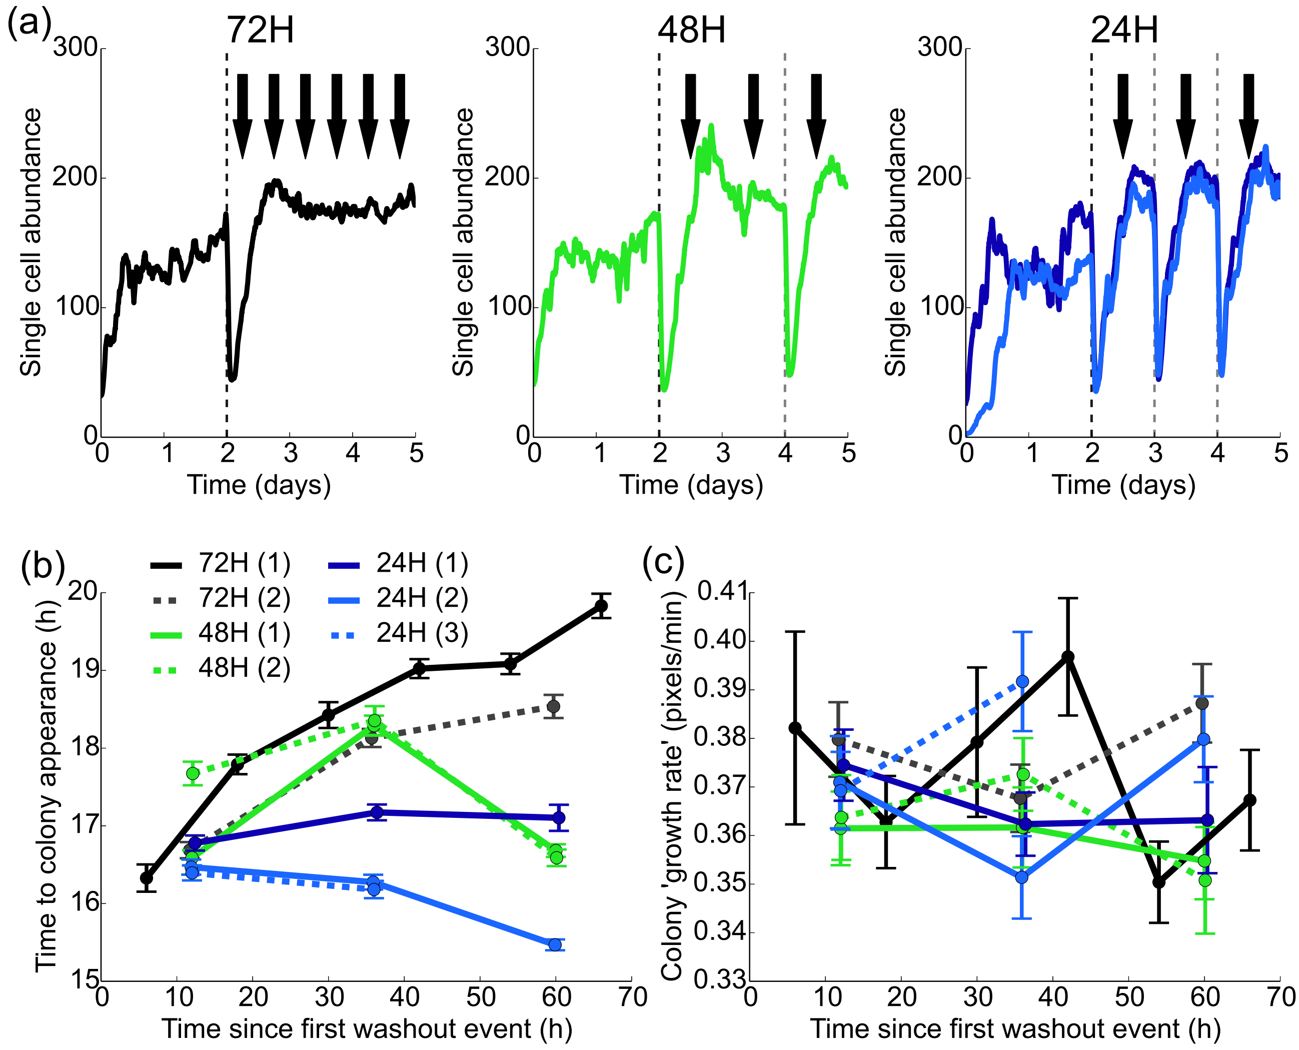


FIG. S2. Lag-phase duration depends on washout event frequency. (a) Single cell abundance (cells per image) time series for four primary data sets. Dashed lines indicate washout events, and arrows indicate time points when sampling occurred. (b) Mean time to colony appearance for populations experiencing 1 h washout events at periods from 72 h to 24 h as a function of time since the first washout events. The legend indicates (period, replicate number). Experiment '24 (3)' ended before the final time sampling point due to computer failure, and experiment '48 (2)' was performed before the plate preparation protocol was finalized and exhibited some signs of resulting aberrations in data due to plates losing moisture through evaporation. Uncertainties indicate standard error of the mean. (c) Mean colony growth rate measurement, using colony rate of area increase over the first 70 minutes of colony detection in webcam images [Fig. S4] as a proxy. Error bars in all panels indicate standard error of the mean.

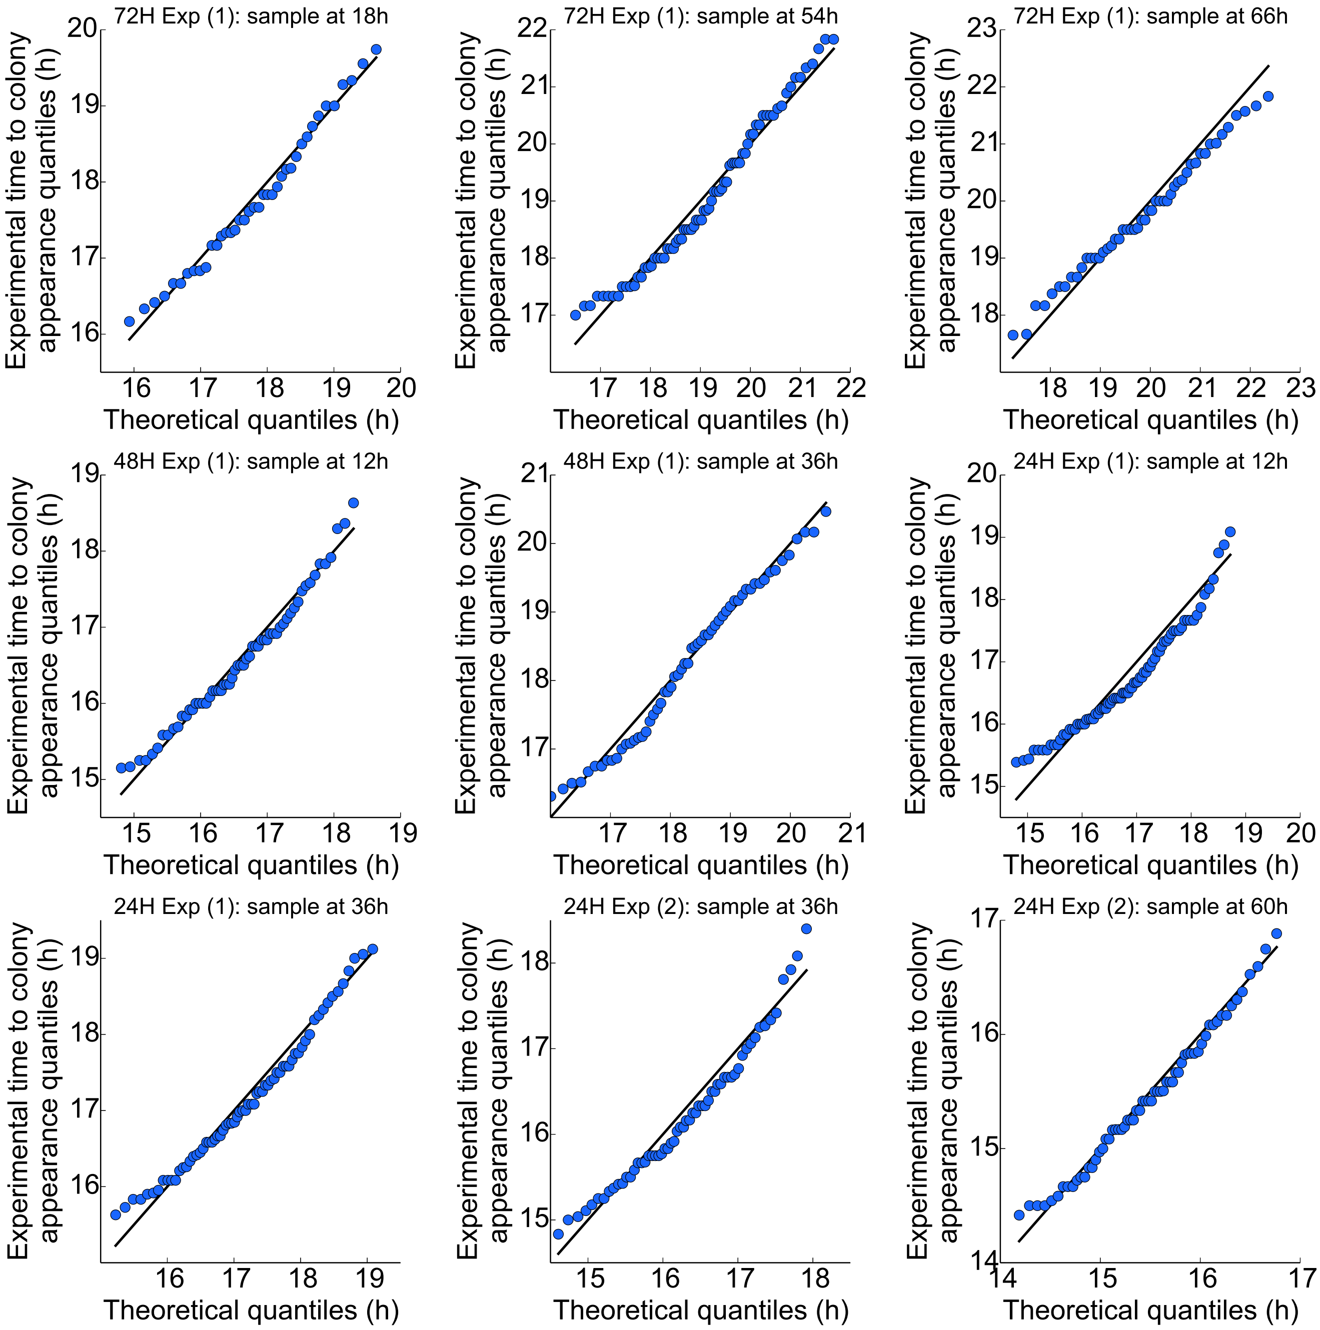


FIG. S3. Lag-phase duration is normally distributed. Quantile-Quantile (qq) plots of time to colony appearance for plates from various time points and experiments in Fig. S2. Each panel includes colonies from two plates. Theoretical distributions are in each case normal distributions with the sample mean and standard deviation from the associated experimental dataset. The black line is a reference representing an experimental distribution perfectly matching a normal distribution; points show the real quantiles of the experimental dataset matched to the quantiles of the theoretical distribution. In each graph, quantiles are evenly spread over the range 0.05 to 0.95.

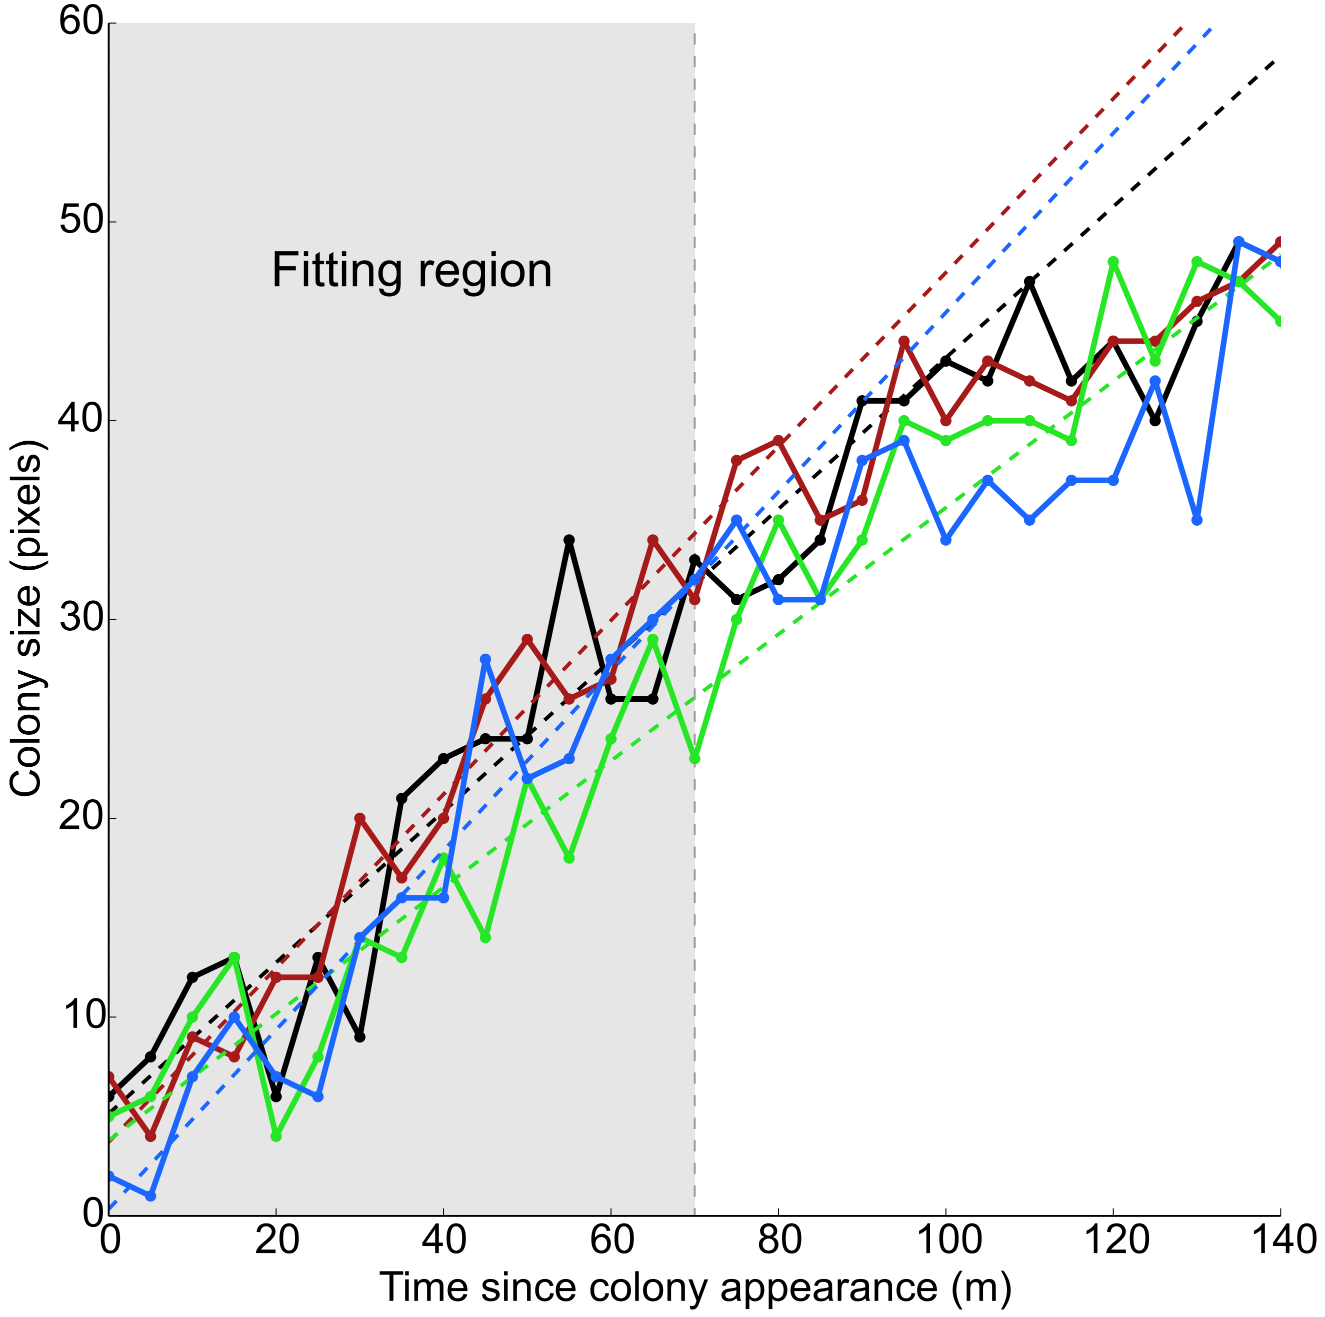


FIG. S4. Colony growth rate measurement. Growth in colony area following initial detection of colony on plates in webcam images for four representative colonies. Colony growth is roughly linear in time over the first 70 minutes.

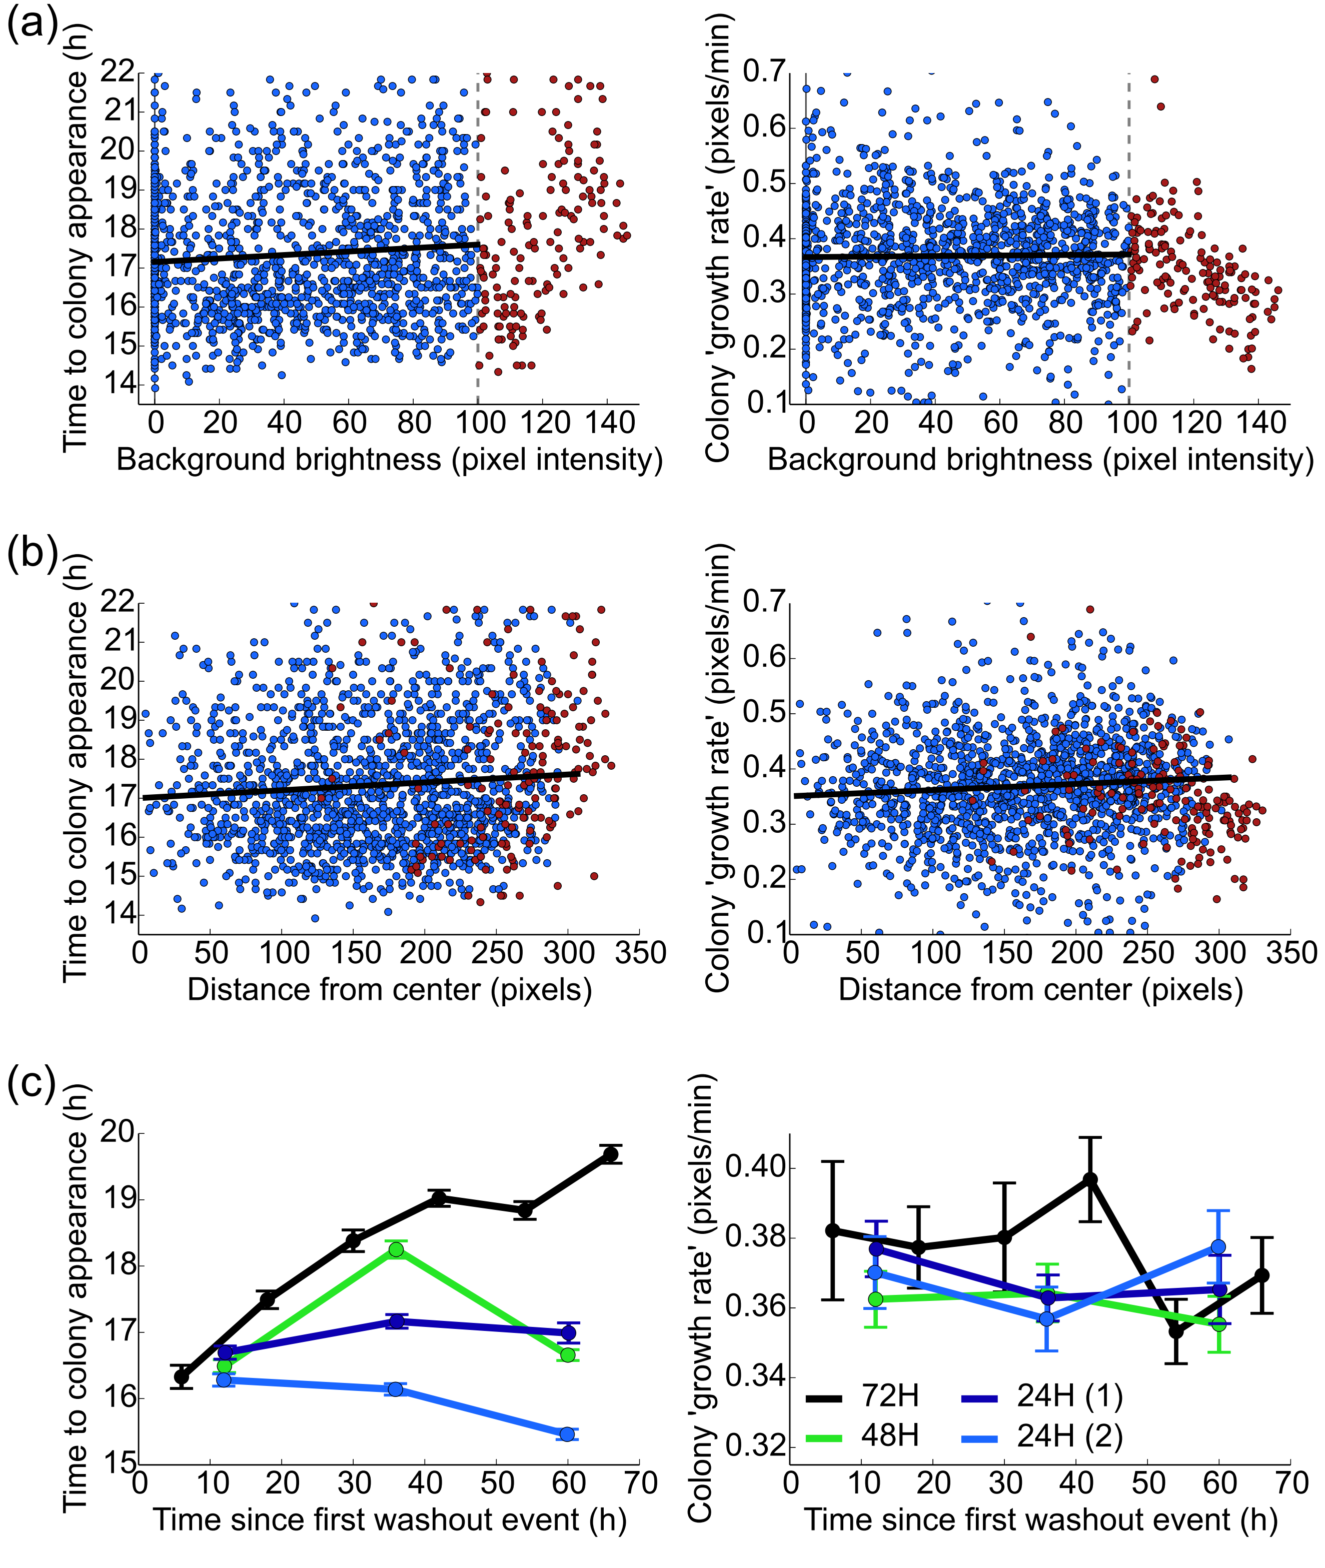


FIG. S5. Effect of background brightness and colony position on measured colony parameters. (a) Time to colony appearance and colony growth rate plotted against background plate brightness at colony location. When the local background brightness exceeds a pixel intensity of 100 it begins to affect the accurate detection and measurement of colonies. Linear fits shown are calculated only over colonies with a background brightness of less than 100, and yield slopes of $(4.45 \pm 1.33) \times 10^{-3}$ h (pixel intensity)$^{-1}$ (left) and $(4.78 \pm 7.99) \times 10^{-5}$ pixels min$^{-1}$ (pixel intensity)$^{-1}$ (right). (b) Time to colony appearance and colony growth rate plotted against distance from center of plate. The location of colonies on the plate has a minor effect on the measured parameters when colonies growing at bright locations are separated out. Linear fits shown are calculated over only colonies with a background brightness of less than 100, and yield slopes of $(2.02 \pm 0.65) \times 10^{-3}$ h pixels$^{-1}$ (left) and $(1.11 \pm 0.39) \times 10^{-4}$ min$^{-1}$ (right). (c) Modified versions of primary data sets from Fig. S2(b),(c) using only colonies below the plate brightness threshold in (a), showing that the qualitative trends are unaffected.

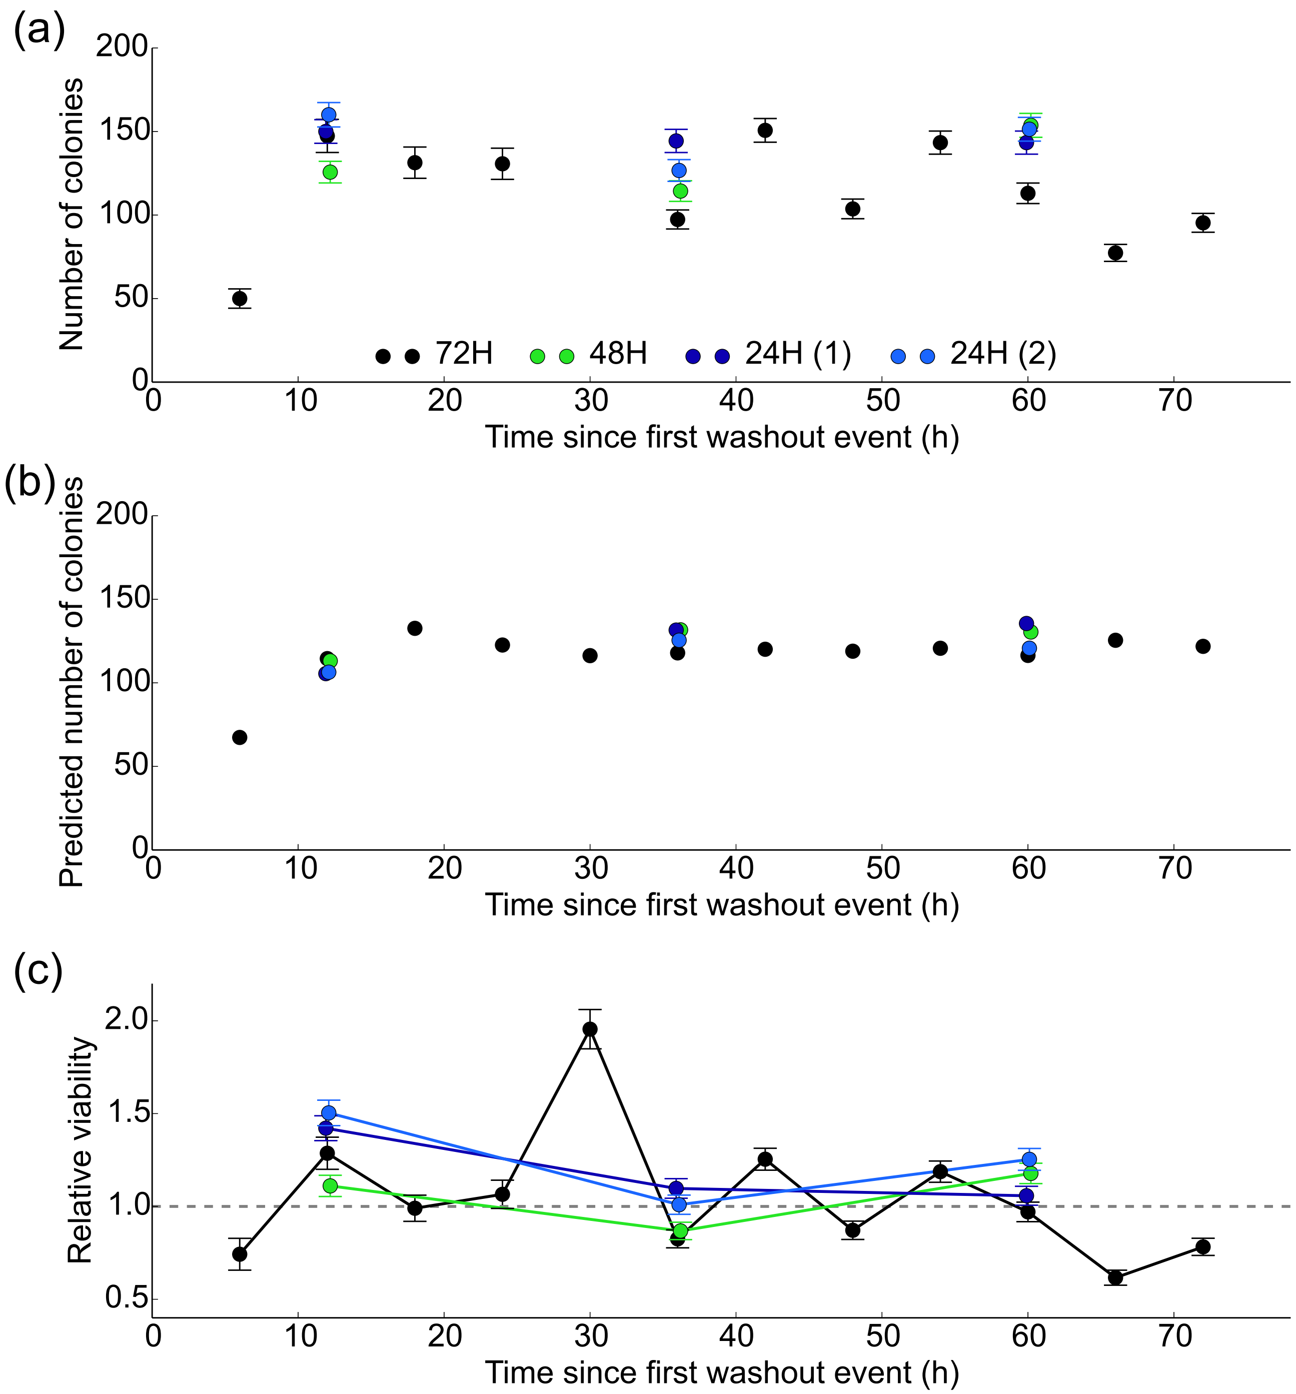


FIG. S6. Cell viability as a function of starvation duration. (a) Average number of colonies counted over three plates by hand from the data sets in Fig. S2(b) plotted with solid lines. The number of colonies per plate in our experiment corresponds to colony-forming units in a 100 µL sample from a $5 \times 10^5$-fold dilution of our system cultures into phosphate-buffered saline. Counts shown here include additional plates not imaged by webcam, as well as additional time points. Note that the total cell abundance in the continuous-culture device is also varying in time as shown in (b) and Fig. S2, and the low number of colonies at the 6 hour time point is predicted by the smaller population in the chemostat at that time. The high number of colonies at 30 hours is attributed to a single plate (not imaged by webcam) with over 4 times the expected number of colonies, possibly the result of inadvertently spreading a cell aggregate over the plate. Uncertainties shown assume Poisson counting error in colony counts. (b) Predicted number of colonies at the sampling time points based on cells per image in microscope data and earlier calibration [2] yielding a conversion factor of 1.48 cells per image corresponding to 1 colony per plate. (c) Relative viability of cells over time, defined as the measured number of colonies divided by the number of colonies predicted by the number of cells per image, showing no decline in cell viability until at least 60 hours after the first washout event.

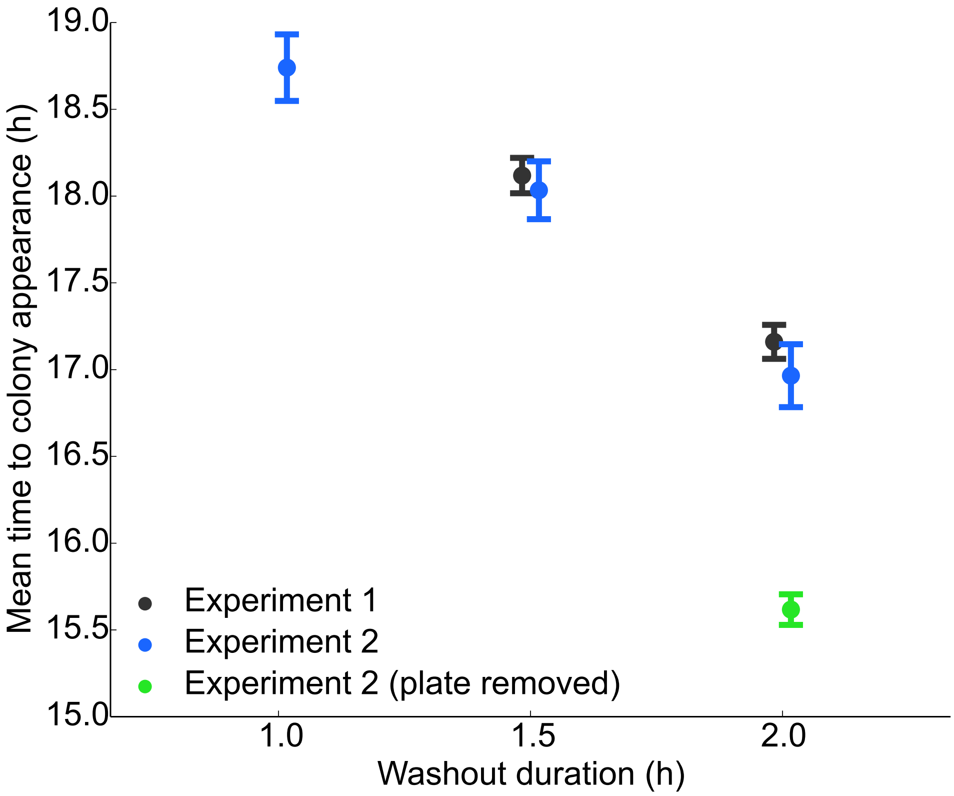


FIG. S7. Lag-phase duration depends on amplitude of washout events. All cells were sampled 12 h following the start of the first washout event in a system which experienced a washout event with duration between 1 h and 2 h. The 'plate removed' data point refers to the removal of a single plate which appeared to have a dramatically different distribution of times to appearance as compared to other plates from the same experiment, most likely due to unexpected evaporation of the plate. Note that due to substantial modifications to the imaging apparatus between experiments, quantitative comparisons to Fig. S2(b) are not valid.

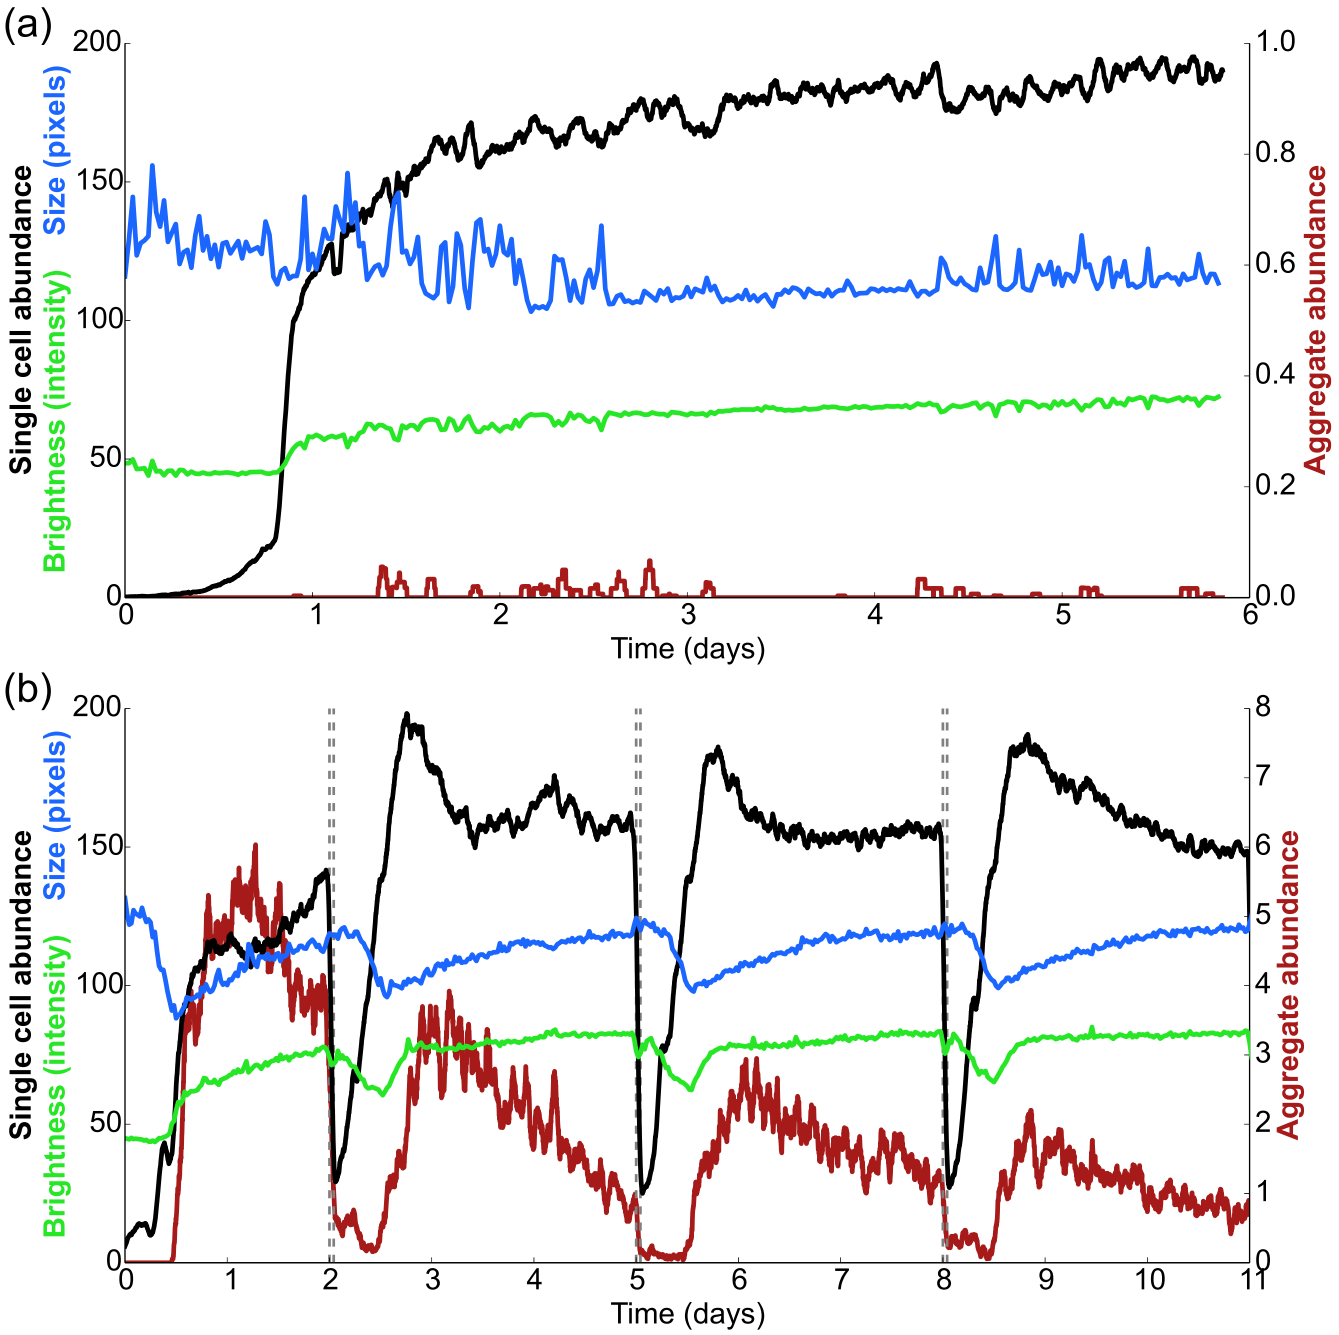


FIG. S8. Dynamics of cell size. Per-image single cell abundance, aggregate abundance, mean cell size (in pixels) and mean cell brightness (in pixel intensity) plotted for (a) a population growing in batch culture ($D = 0$) and (b) a continuous-culture system with a washout event schedule of 72 hours. Axis label colors correspond to colors of traces. Single cell and aggregate abundances are each smoothed with a 1 hour rolling average. Cell size decreases in batch culture but increases in continuous-culture even in starvation conditions; a cell size of 100 pixels corresponds roughly to an area of $3.1\,\mu m^2$ in the focal plane. Pixel intensity is in the range 0-255, and the population mean cell brightness is calculated as a population average over the mean brightness of each individual cell. Note that the apparent spike in cell abundance prior to $T = 1\,d$ as the pixel intensity increases above 50 is an artifact due to population brightness increasing to the point all cells are detected. Prior to this sudden increase, only bright cells are counted; after the increase, cells remain bright enough to be correctly segmented for the remainder of the experiment in all continuous-culture conditions.

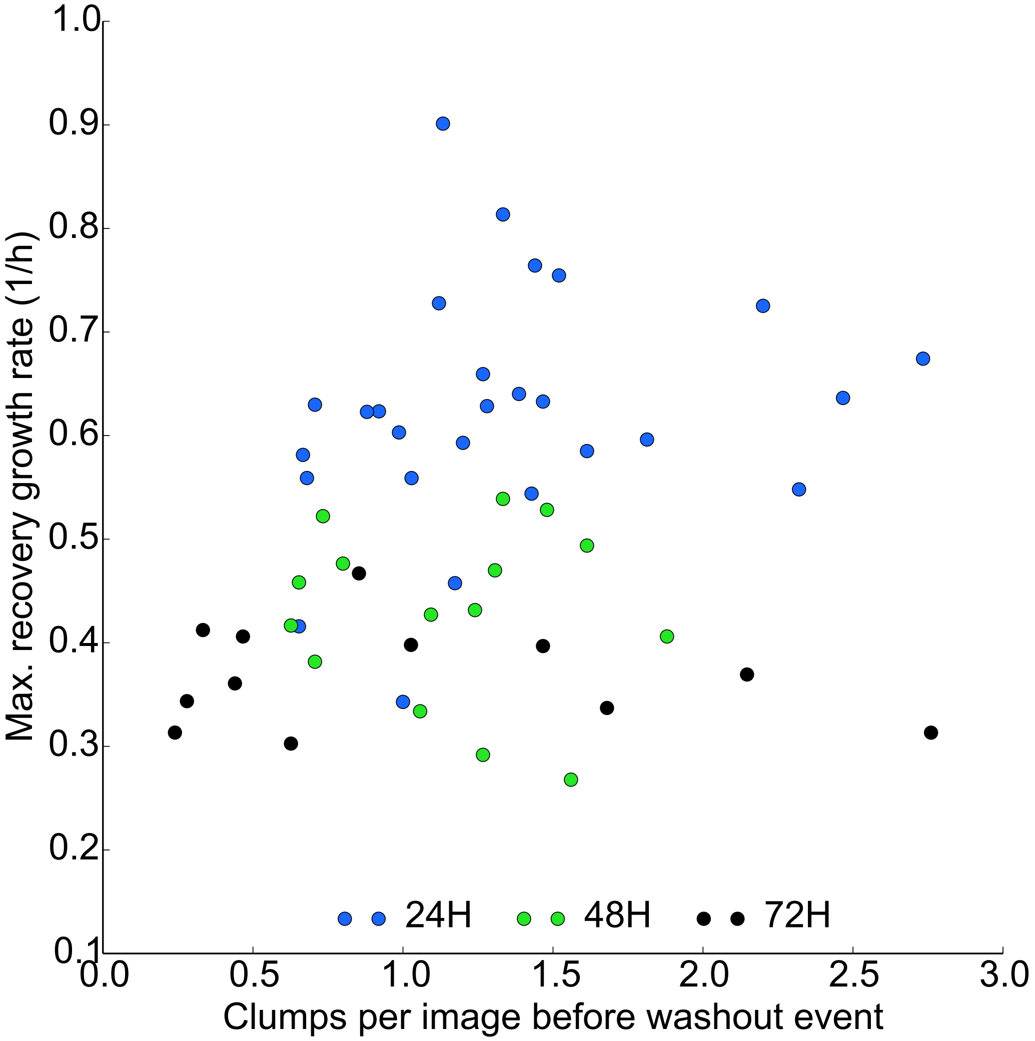


FIG. S9. Number of aggregates prior to washout event plotted against spline-estimated maximum growth rate during recovery in 1 h washout event conditions. The number of aggregates prior to a washout event is estimated by an average over 15 minutes of data immediately before the washout event.

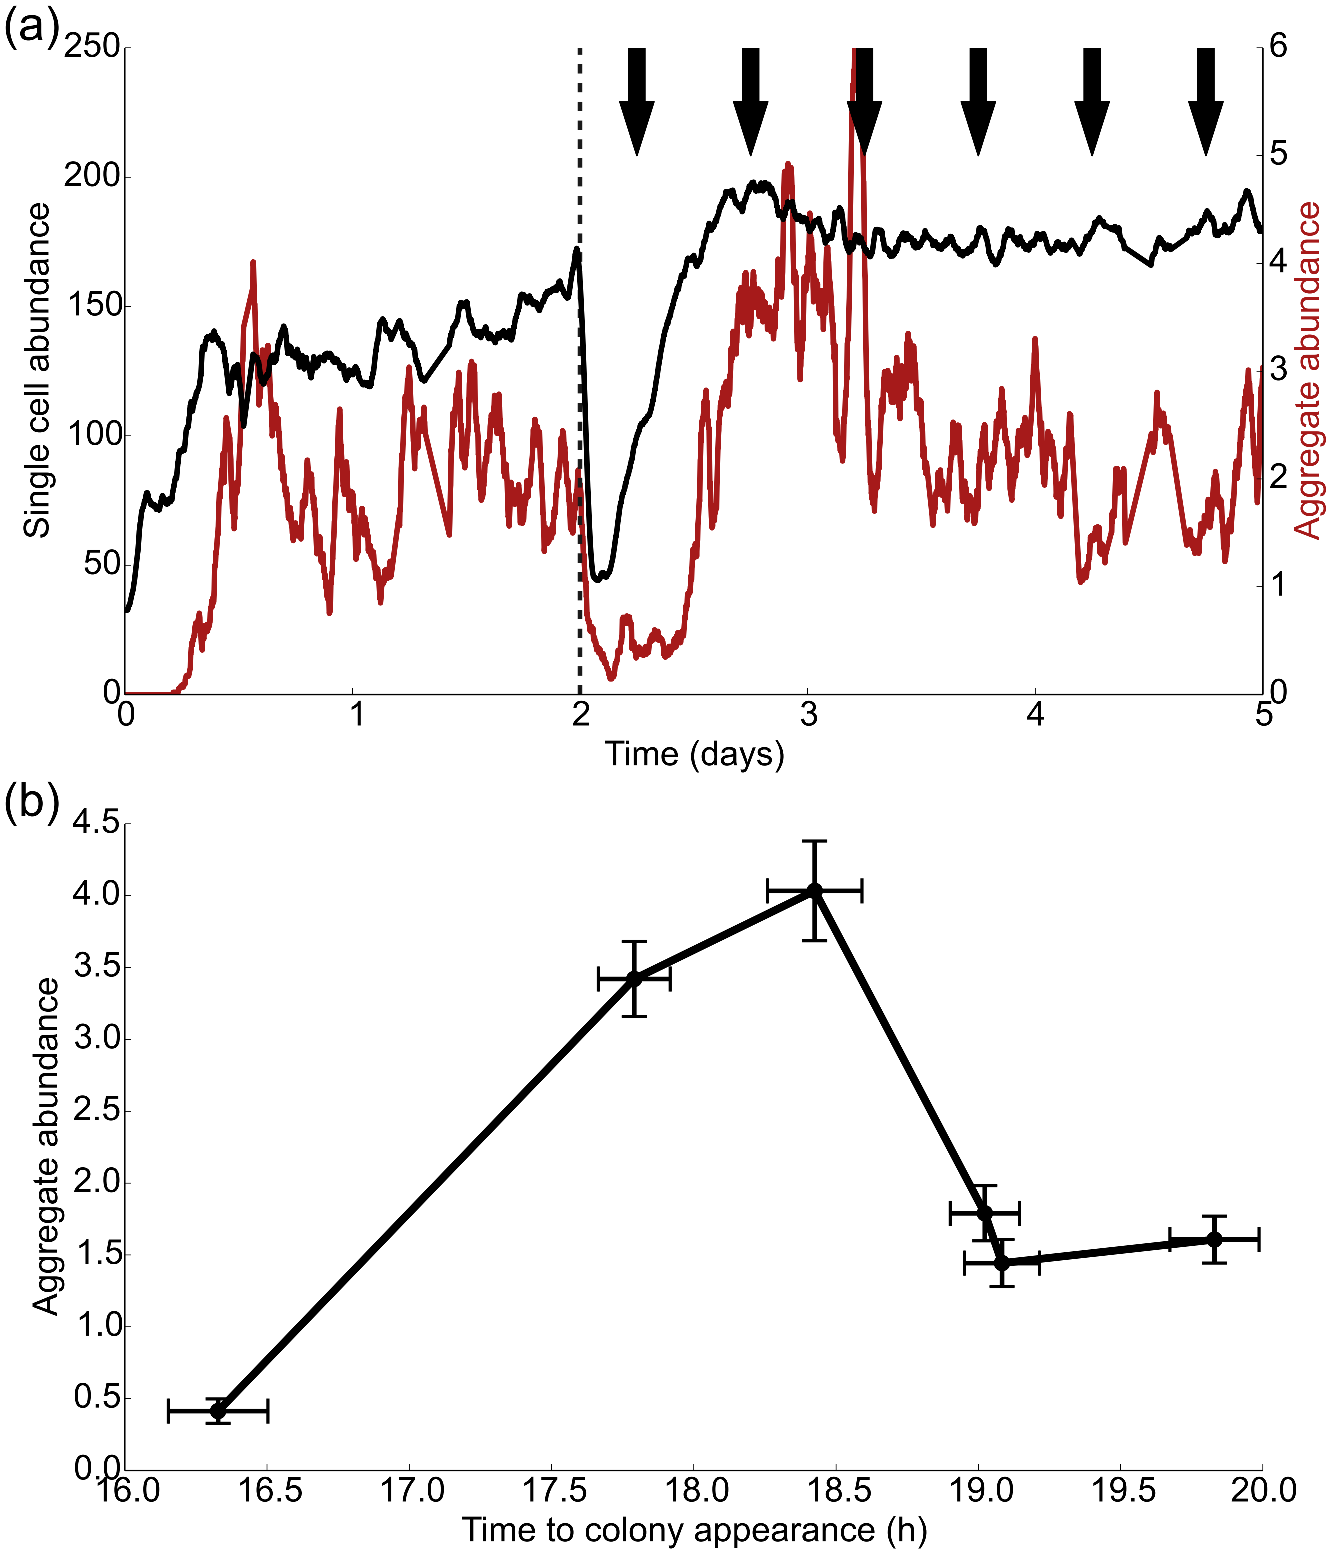


FIG. S10. (a) Single cell and aggregate per-image abundances during the 72 h experiment shown in Fig. S2(a). Single cell and aggregate abundance are each smoothed with a 1 hour rolling average. Black arrows indicate sampling times. (b) Number of aggregates vs. mean single-cell lag time, using time to colony appearance on plates in webcam images as a proxy for lag time. Number of aggregates shown is averaged over one hour of data centered on the sampling time. The time to colony appearance is monotonic increasing with sampling time, and the variation in aggregate abundance shows the growth and decline of the aggregate population following recovery from a washout event, similar to the experiment shown in [Fig. S8(b)]. Indicated uncertainties are standard error of the mean.

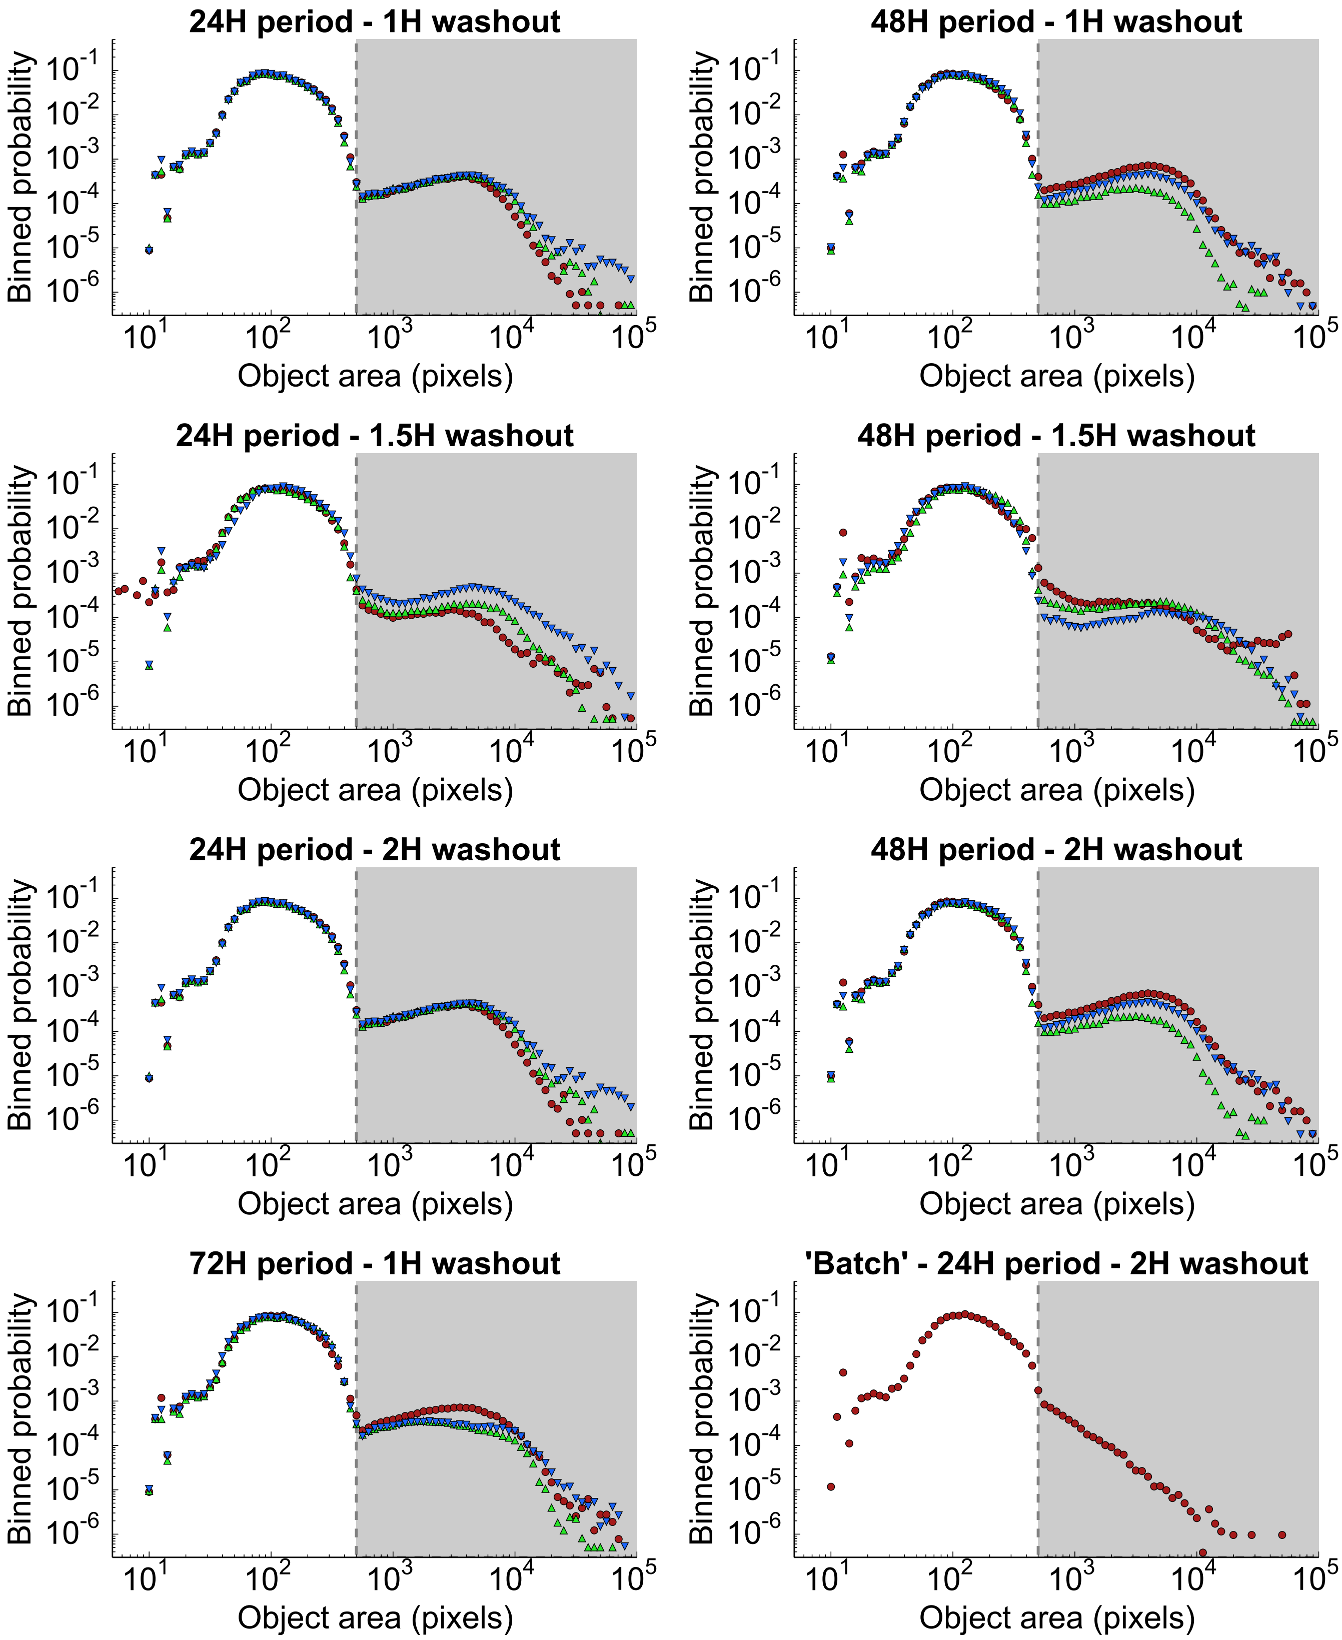


FIG. S11. Binned probability histograms of sizes of all objects detected during image segmentation under different experimental conditions over the 9 day experiment window, with logarithmic bins of object area and each bin normalized by the total number of objects. Two distinct peaks in the distribution are clear under continuous-culture conditions, corresponding to the most common size ranges for single cells and aggregates, whereas in a batch experiment no higher mode of the distribution is observed. We note that to prevent double-counting of bright cells, because the tail of the distribution of single-cell sizes drops off rapidly by approximately 500 pixels (indicated by the dashed line), the aggregate image segmentation routine does not detect objects below 500 pixels in size. As a result, all objects shown here in unshaded regions are classified in abundance time series as single cells, and the vast majority of objects shown here in shaded regions are classified as aggregates.

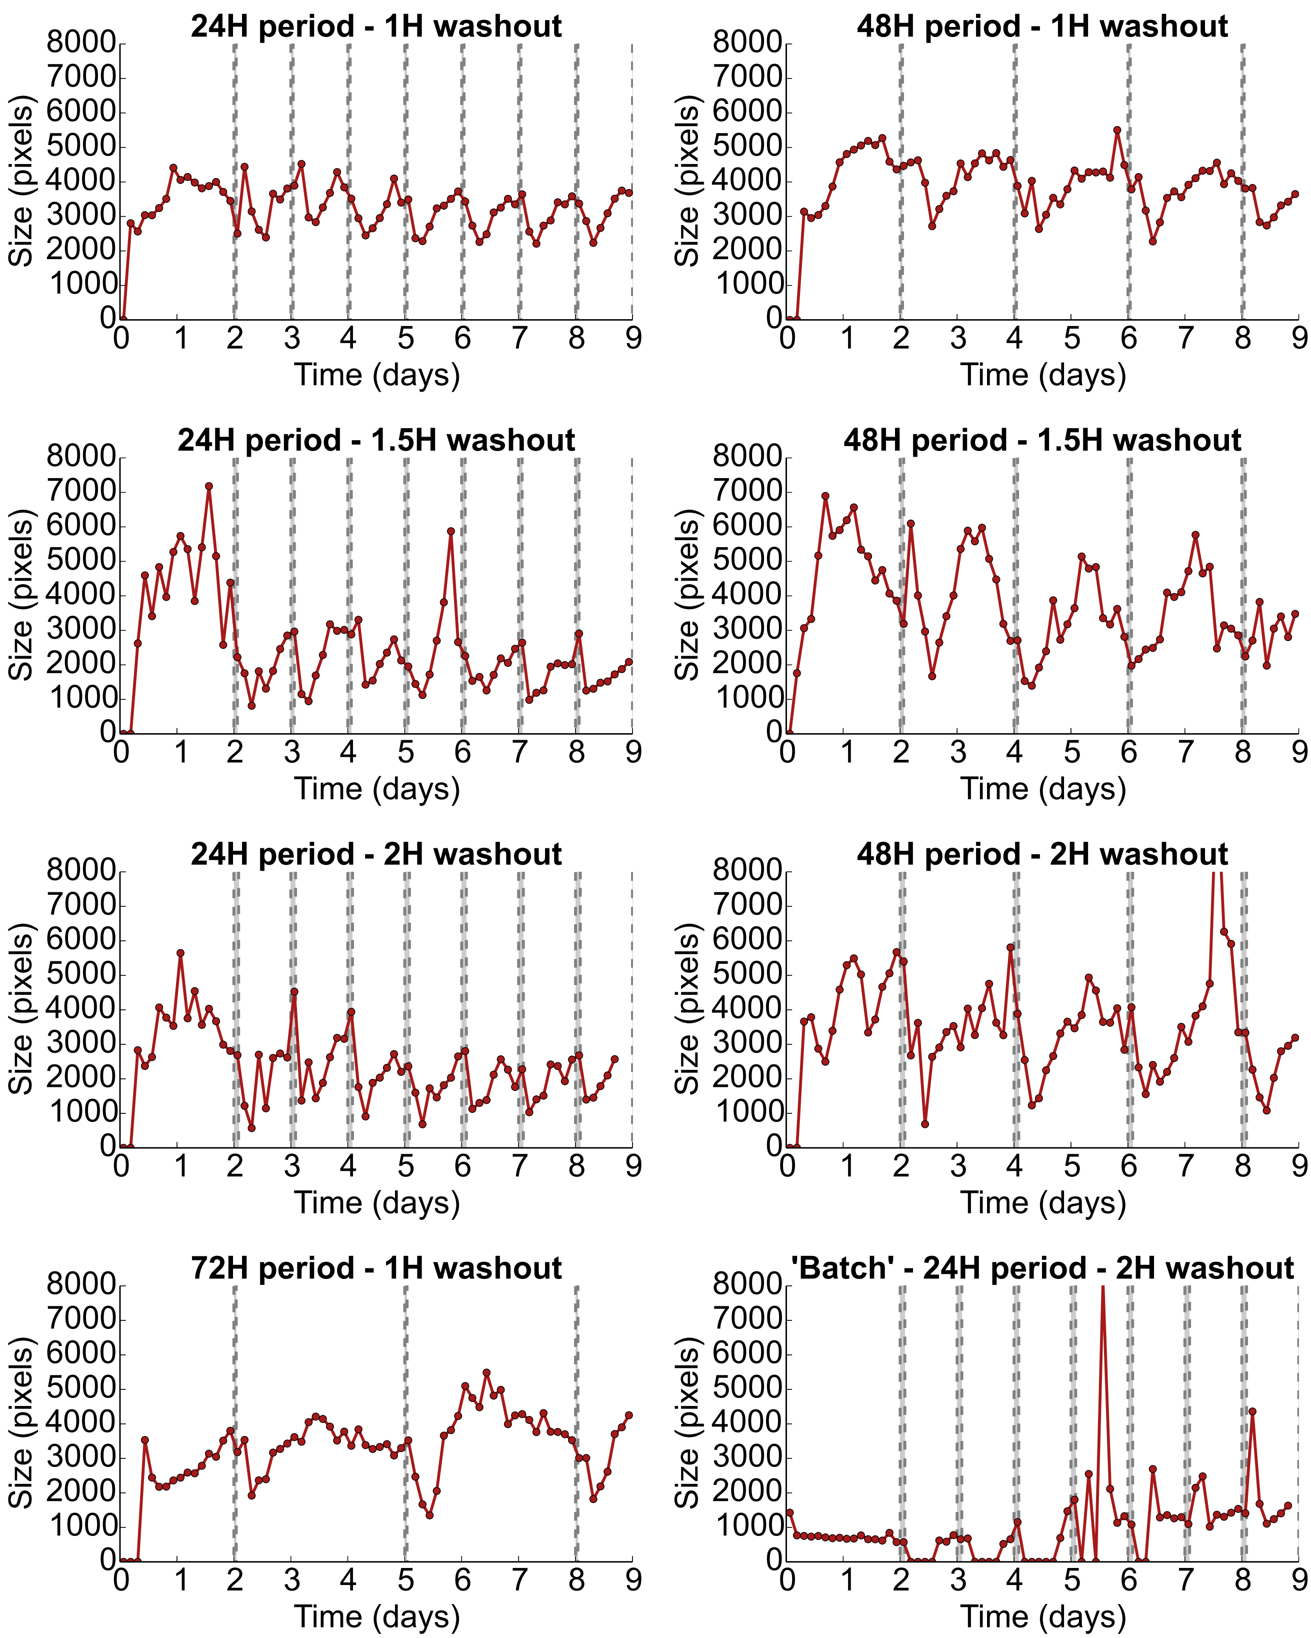


FIG. S12. Aggregates decrease in size after washout events. Binned time series (3 hour windows) of average aggregate sizes across different experimental conditions, showing a rapid decrease in aggregate size following a washout event, followed by a steady increase, with additional dynamics present in systems with long washout periods. Shaded regions indicate washout events, and an average aggregate size of zero indicates the absence of aggregates. Note that the increase in aggregate size in the 'batch'-style experiment from between days 5 and 6 correlates to the rise in aggregate population in that experiment shown in Fig. S15(b) and a rise in the observed maximum recovery rate by optical density as shown in Fig. S15(c).

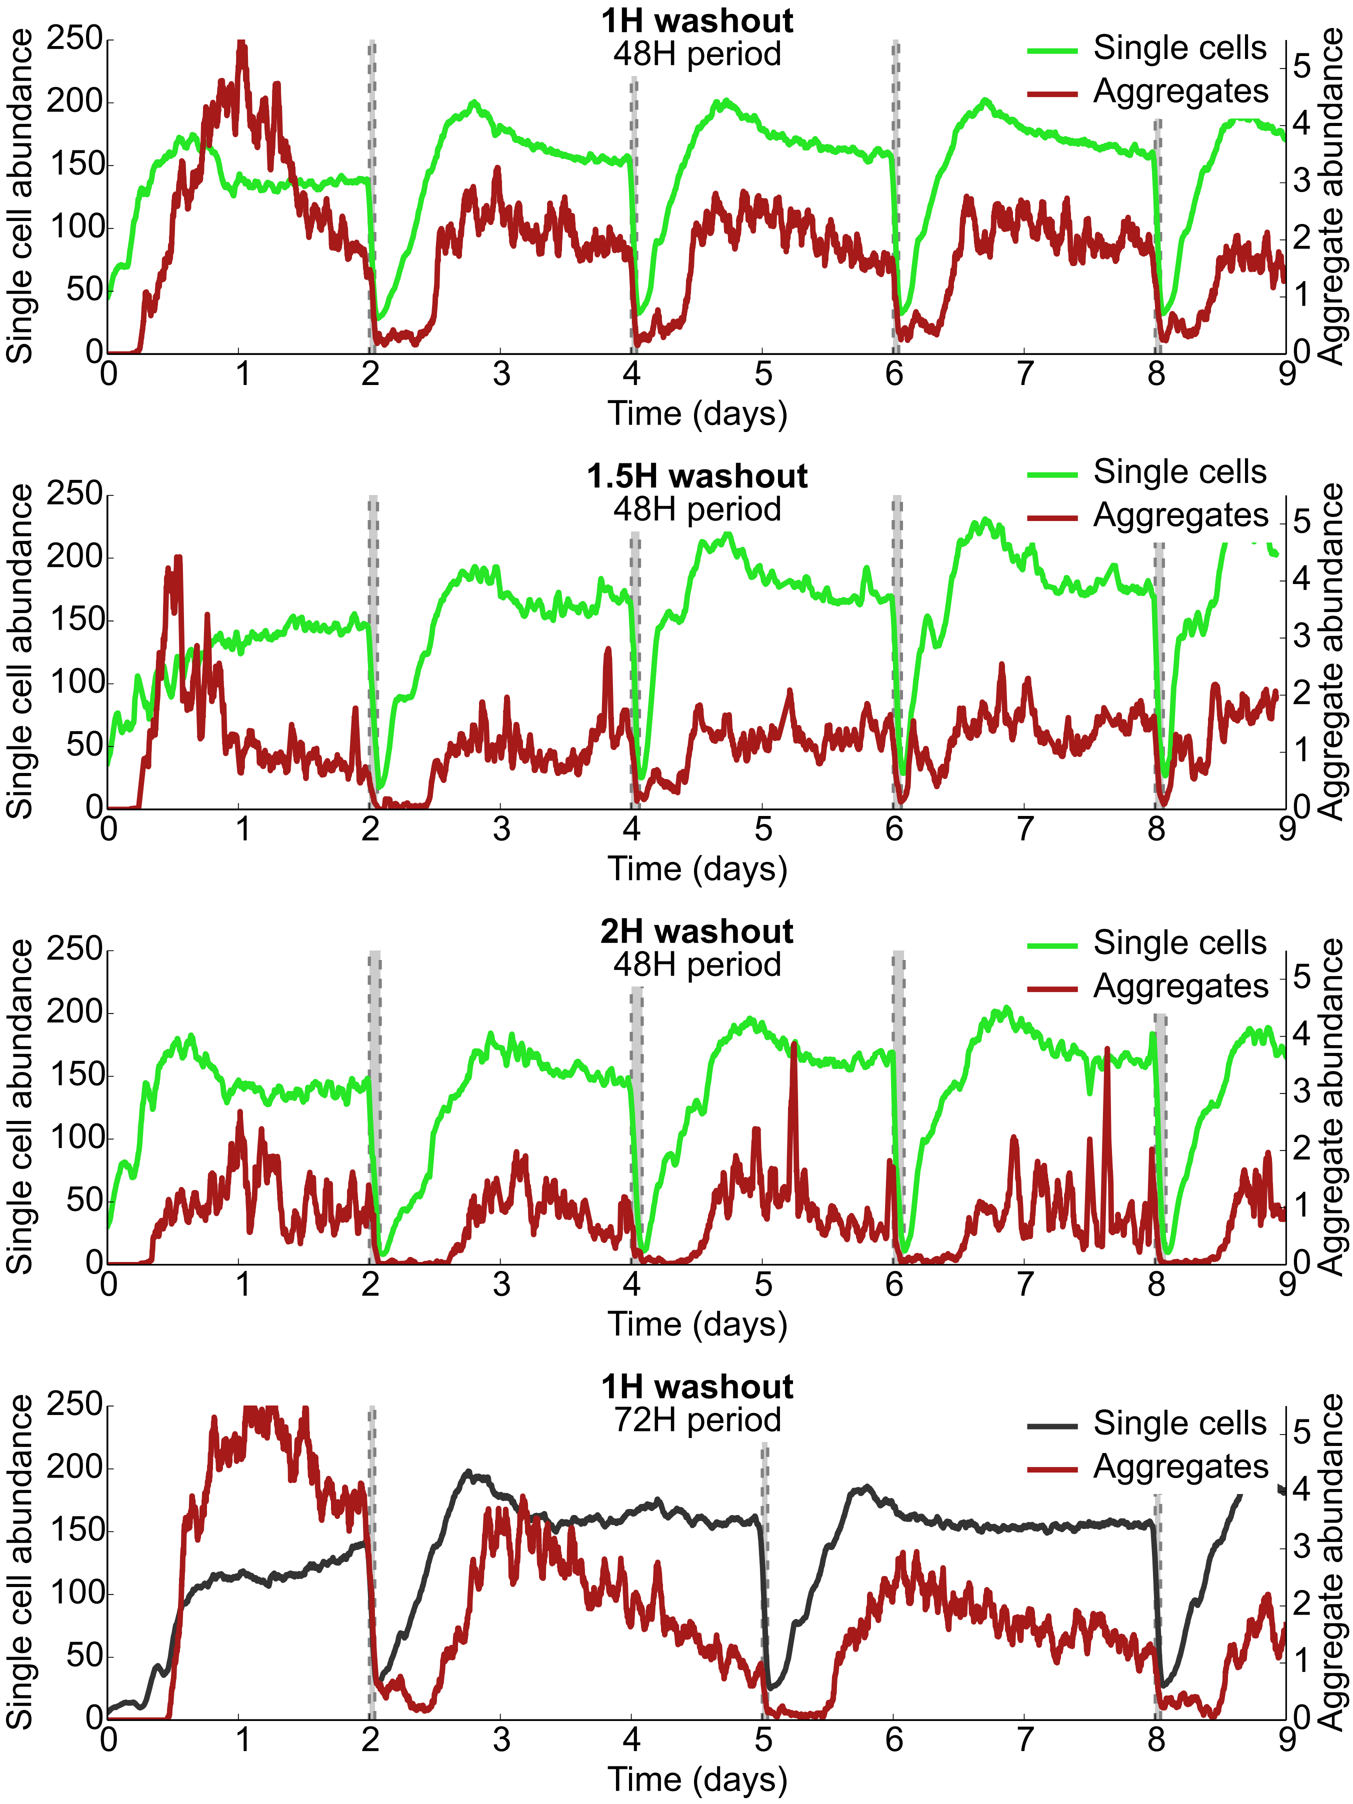


FIG. S13. Example per-image abundance dynamics of single-cell populations and aggregates under washout conditions not shown in the main text. Single-cell and aggregate abundances are each smoothed with a 1 hour rolling average. Shaded regions indicate washout events.

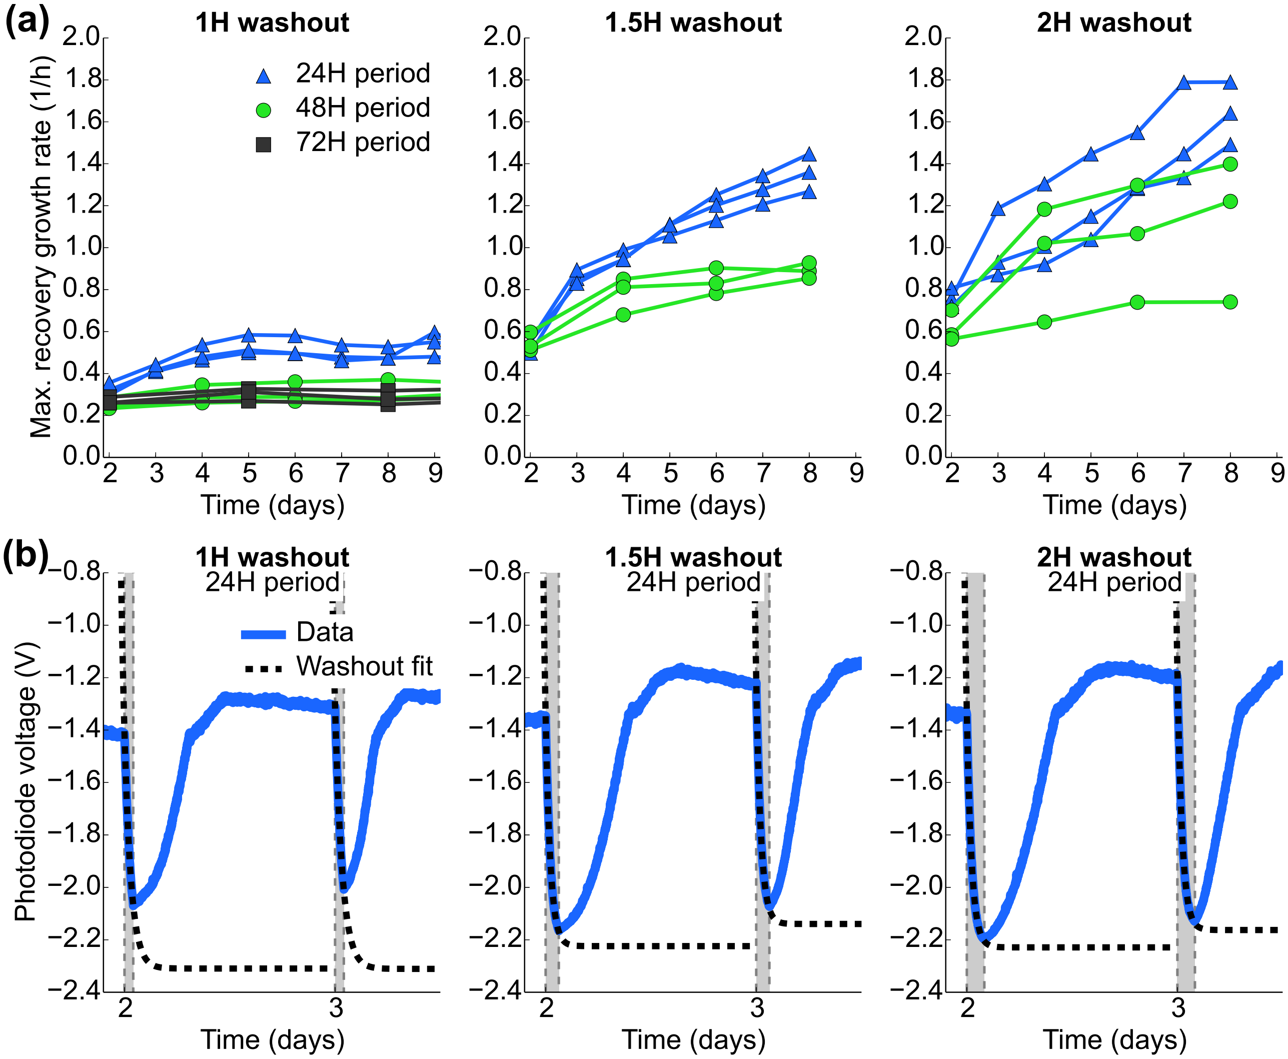


FIG. S14. Frequency and amplitude dependent dynamics measured by optical density. (a) Estimated maximum population growth rates during recovery for 1 h, 1.5 h and 2 h washouts, based on optical density measurements alone, at different washout frequencies. (b) Representative optical density time series for one replicate each from experiments with 1 h, 1.5 h, and 2 h washouts, all with a 24 h washout period. Dashed lines indicate the decaying exponential fits to washout data used to determine the system 'zero' for optical density during the following recovery. Shaded regions indicate washout events.

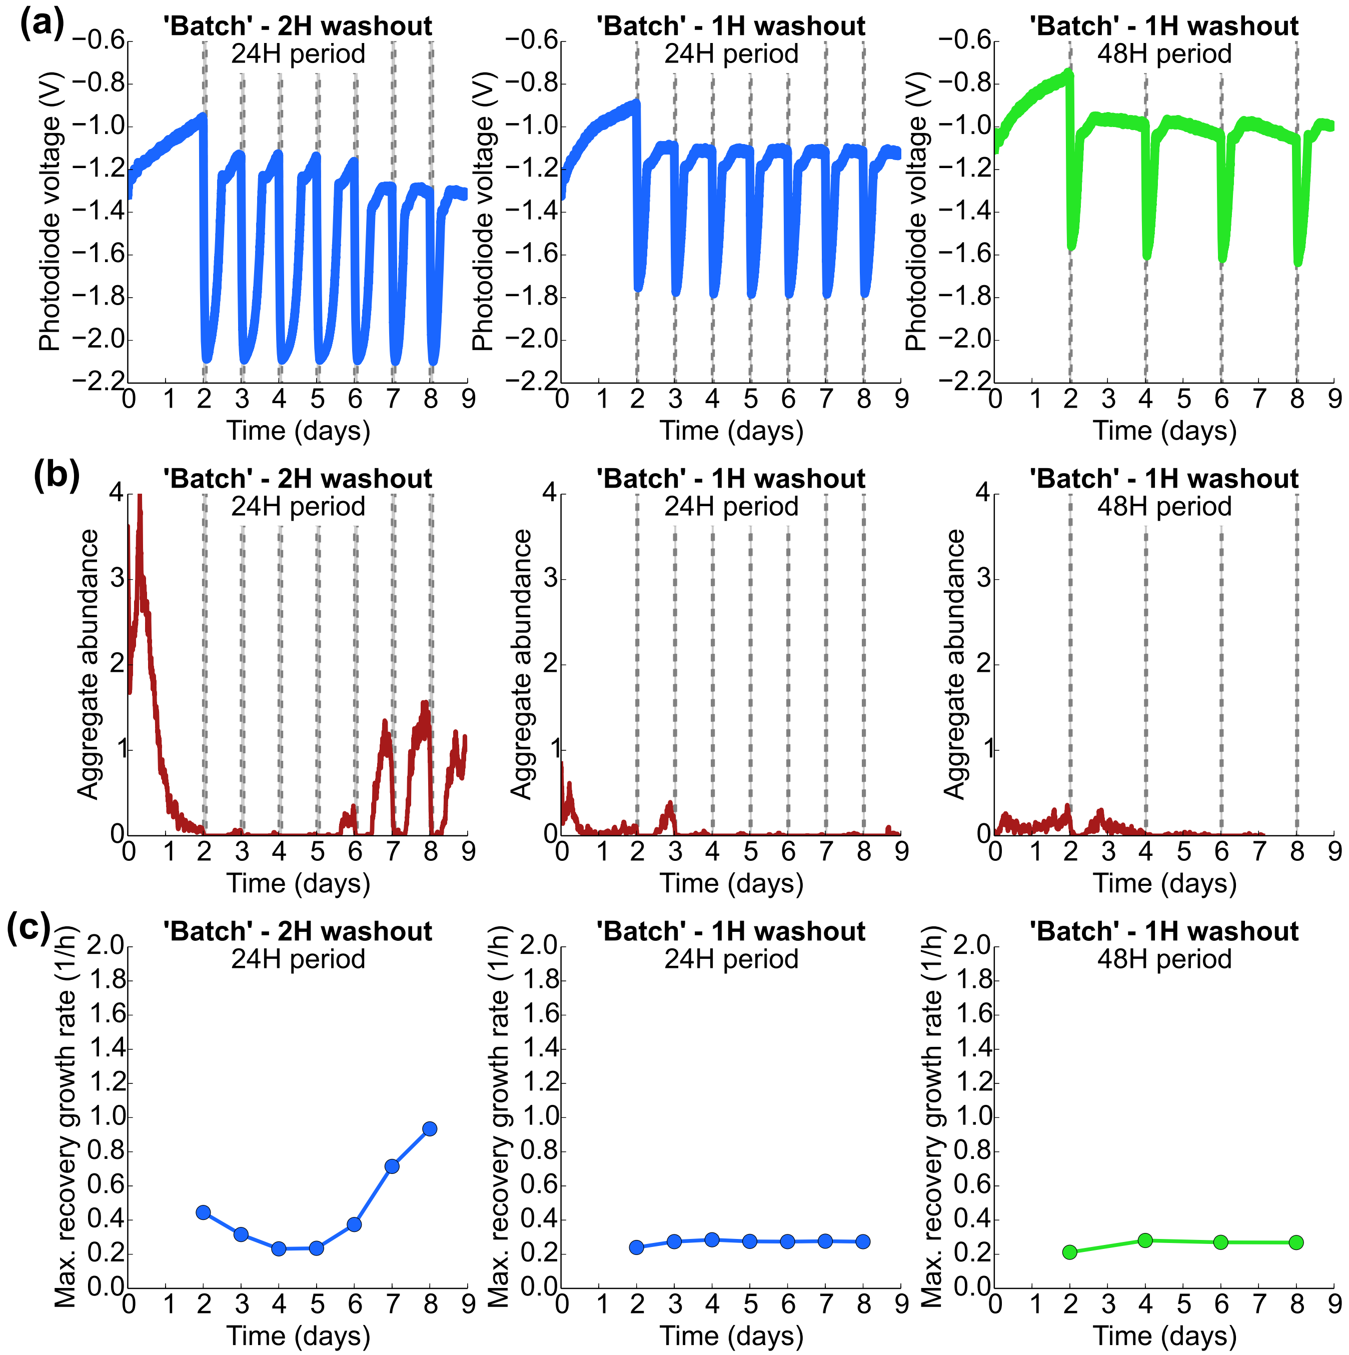


FIG. S15. Batch-style experiment show no frequency or amplitude dependence. (a) Optical density time series of ‘batch’-style experiments ($D = 0$ between washout events). Shaded regions indicate washout events. (b) Cell aggregate abundance (per image) time series, as determined by standard image processing. As the camera exposure time was increased substantially for these experiments, the brightness threshold for detection of aggregates was slightly increased to filter out uncommonly bright single cells. We note the eventual appearance of aggregates in the 2 h washout condition, correlated with a size increase in detected aggregates as shown in Fig. S12. (c) Maximum optical density recovery rates based on data shown in (a). We note that these do not show the strong frequency-dependence and amplitude-dependence of our continuous-culture experiments, shown in Fig. S14(a) and Fig. 2(a), but that the recovery rate does eventually begin to increase in the 2 h washout condition, correlating in time with the appearance of aggregates.

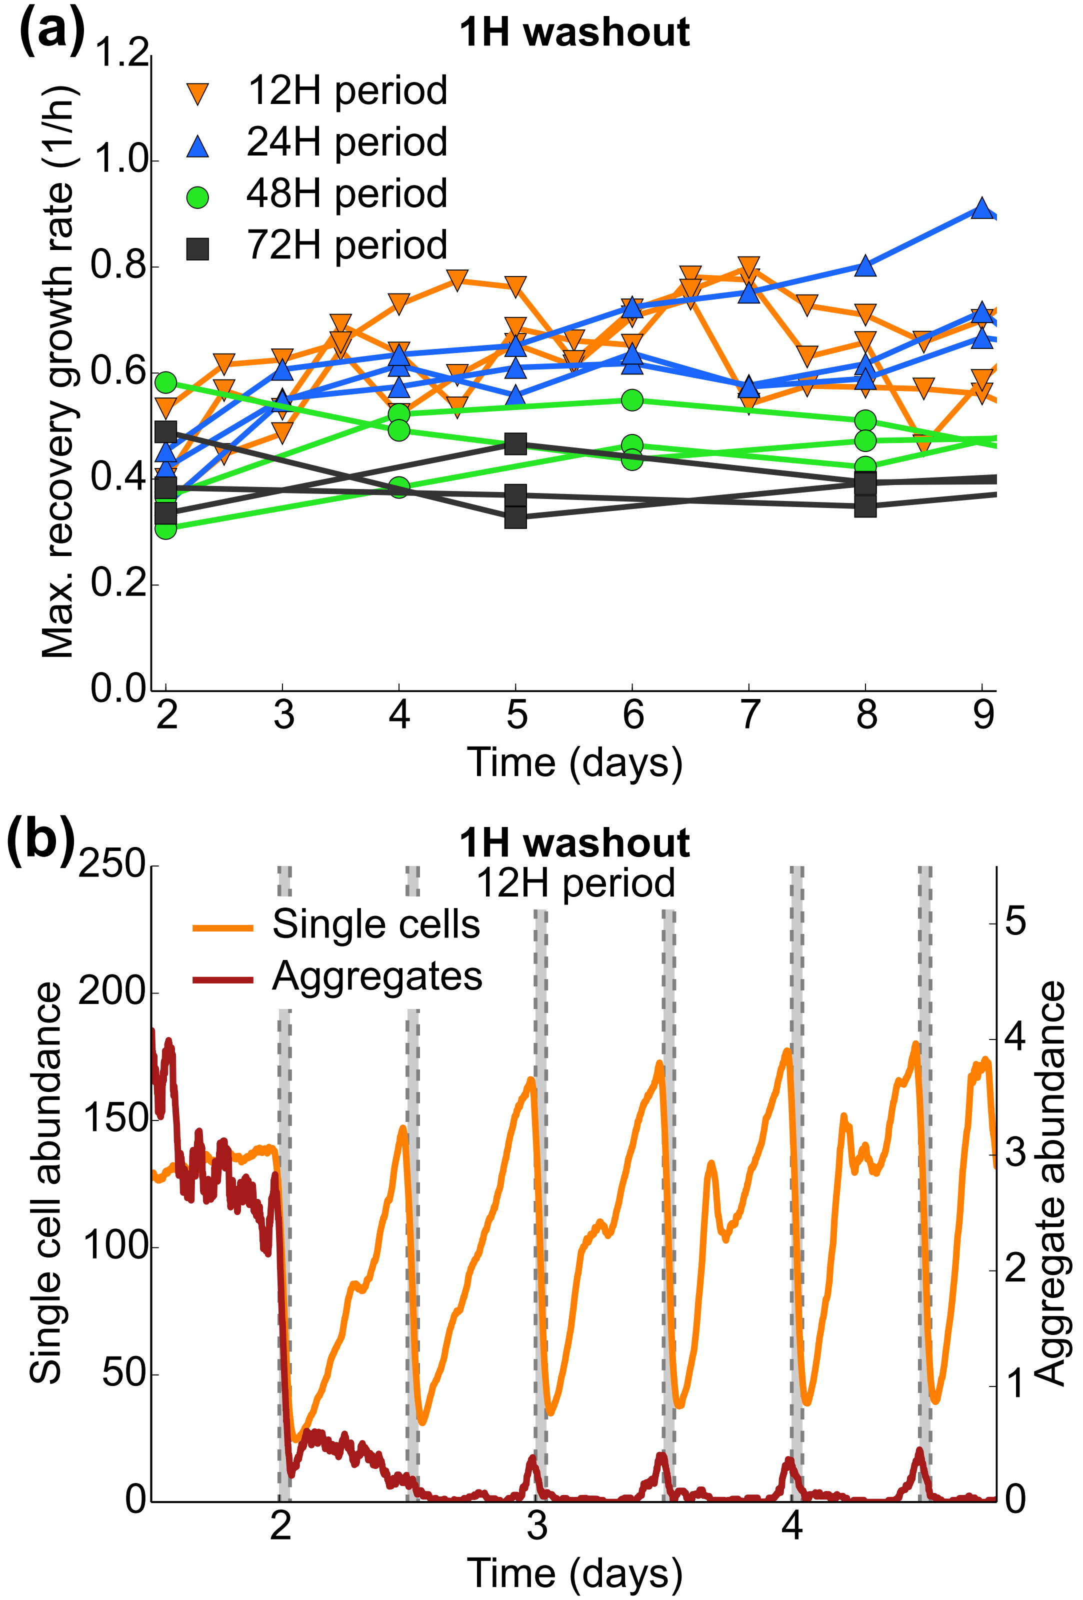


FIG. S16. High frequency abundance dynamics. (a) Maximum recovery rates from 1 h washout experiments, with high-frequency 12 h washout period included. (b) Single-cell and aggregate abundance (per image) time series, each smoothed with a 1 hour rolling average, from a 12 h washout period replicate. Shaded regions indicate washout events. Fast recovery washouts are maintained despite the low abundance of detected cell aggregates.

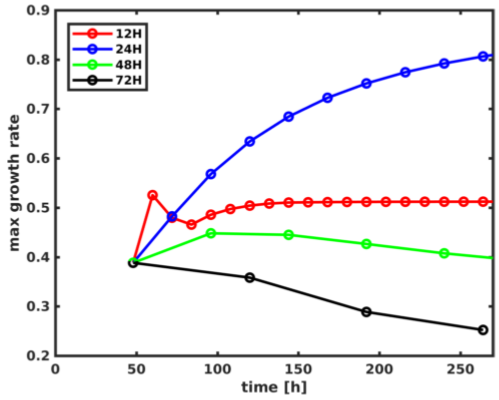


FIG. S17. Simulations do not capture maximum per-hour recovery rate dynamics expected from experiment [Fig. S16(a)] in high frequency 12 h washout schedule with 1 h washout duration.

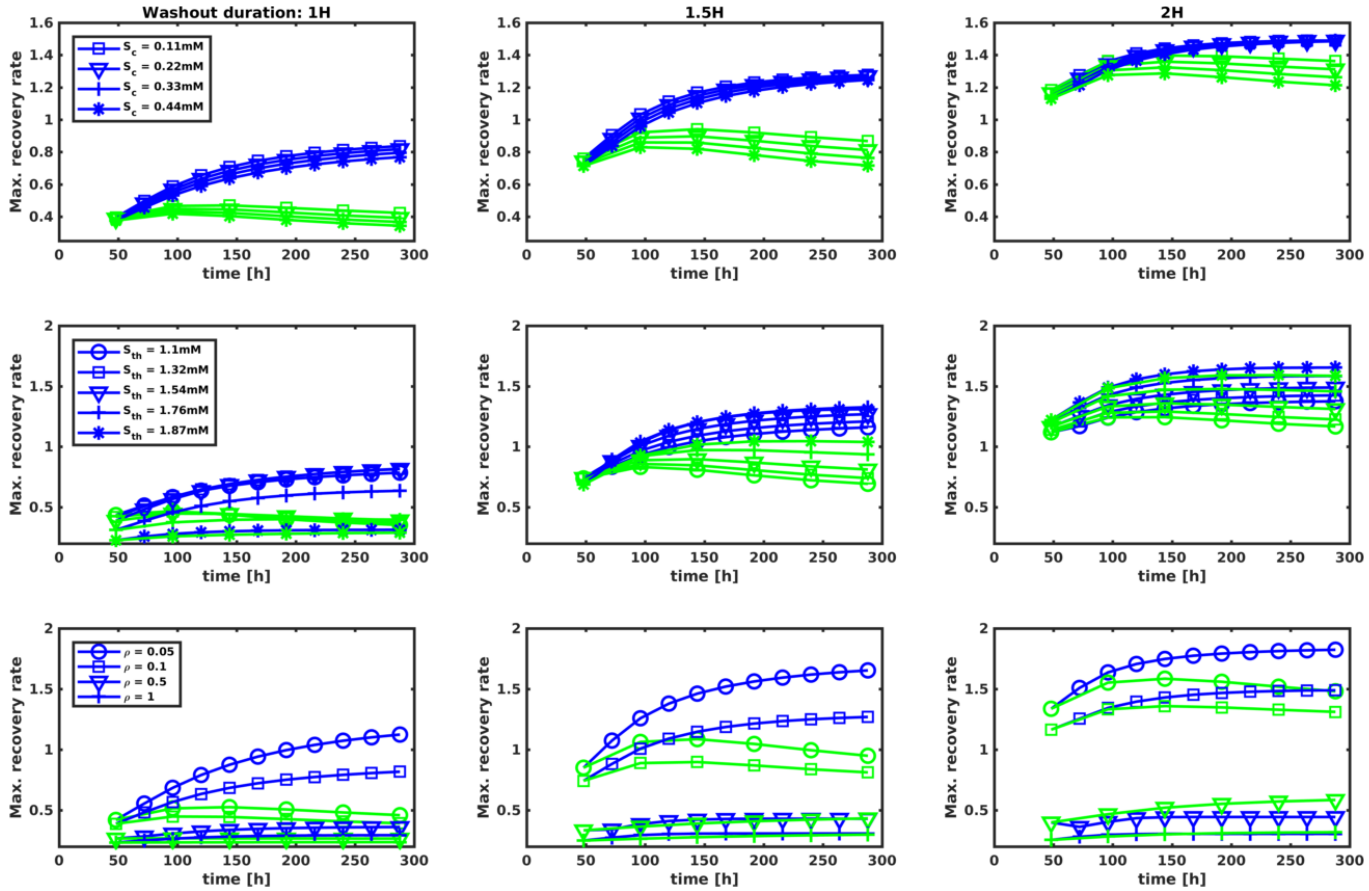


FIG. S18. Simulations of maximum per-hour recovery rates with variable parameters. Three parameters were systematically varied to determine the sensitivity of our conclusions to chosen parameter values. Each row corresponds to a different parameter: $S_c$ (top), $S_{th}$ (middle), $\rho$ (bottom). Each column corresponds to a washout event duration: 1 h (left), 1.5 h (middle) and 2 h (right). Within each panel blue traces correspond to a 24 h washout event schedule and green traces to a 48 h washout event schedule. Different symbols (□, ∘ etc) correspond to different parameter values as denoted by the legends in the left column. Green and blue traces with the same symbols are simulations with the same value of the relevant parameter. For example, in the lower right panel the blue and green traces plotted with ∘ are 24 and 48 hour conditions with $\rho = 0.05$. The values of $S_{th}$ and $S_c$ should be considered relative to the reservoir glucose concentration, $S_r = 2.2$mM.

[1] I. Levin-Reisman, O. Gefen, O. Fridman, I. Ronin, D. Shwa, H. Sheftel, and N. Q. Balaban, Nat. Methods **7**, 737 (2010).
[2] J. Merritt and S. Kuehn, Sci. Rep. **6**, 33173 (2016).
[3] M. Scott, C. W. Gunderson, E. M. Mateescu, Z. Zhang, and T. Hwa, Science **330**, 1099 (2010).
[4] H. Senn, U. Lendenmann, M. Snozzi, G. Hamer, and T. Egli, Biochim. Biophys. Acta **1201**, 424 (1994).
[5] A. Ito, T. May, K. Kawata, and S. Okabe, Biotechnol. Bioeng. **99**, 1462 (2008).
